# Supplementary material for: Chiral excitonic systems in twisted bilayers from F\"{o}rster coupling and unconventional excitonic Hall effects
Source: arXiv:2406.09674 source file (2024-06-20)
Supplement: Supplementary file 1 [file Supp.pdf]

# Supplementary: Nontrivial twisted bilayer chiral excitonic systems: Förster coupling and related Hall effect

Ci Li[1] and Wang Yao[2,3,*]

[1]*School of Physics and Electronics, Hunan University, Changsha 410082, China*

[2]*New Cornerstone Science Laboratory, Department of Physics, University of Hong Kong, Hong Kong, China*

[3]*HKU-UCAS Joint Institute of Theoretical and Computational Physics at Hong Kong, China*

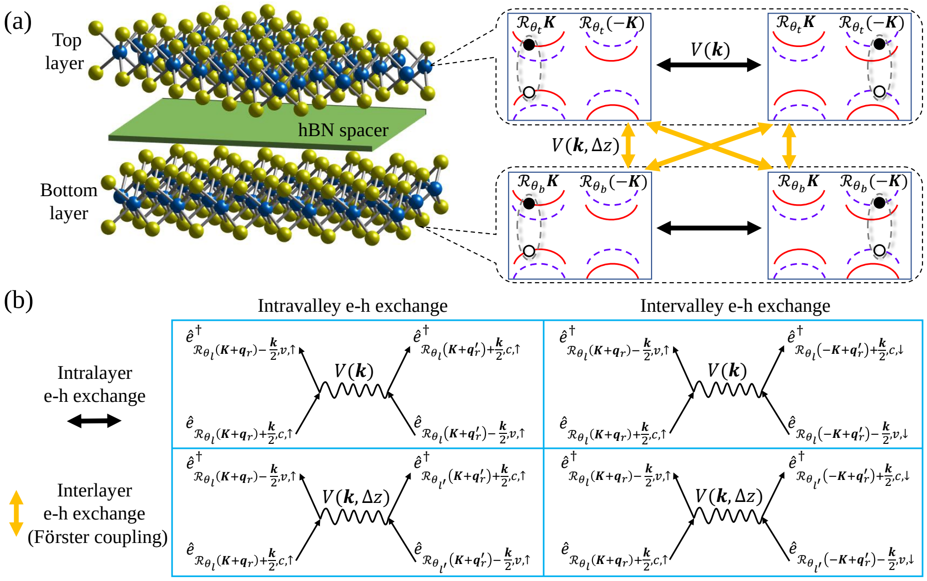


FIG. S1. (color online)(a) Schematic of an arbitrarily twisted homobilayer TMDs as an example, where hBN spacers quench the charge hopping. The intralayer electron-hole (e-h) Coulomb exchange (black arrows) couples the two valley configurations of bright excitons in each layer. The Förster coupling (green arrows), i.e., the interlayer e-h exchange, couples bright exciton states from different layers. $\mathcal{R}_{\theta_l}$ is the rotational matrix in momentum space with twisted angle $\theta_l$, where $l, l' = t, b$ for top or bottom layer, and $l \neq l'$. (b) Illustration of intra- and intervalley e-h exchange interactions within the same layer (intralayer e-h exchange) or between different layers (interlayer e-h exchange). This is depicted in terms of the conduction and valance states of electrons. For intralayer e-h exchange, the conduction-band electron in $\mathcal{R}_{\theta_l}K$ valley is scattered to the valence state in the same valley, while the valance-band electron in $\mathcal{R}_{\theta_l}K/\mathcal{R}_{\theta_l}(-K)$ valley is scattered to the conduction state in valley $\mathcal{R}_{\theta_l}K/\mathcal{R}_{\theta_l}(-K)$. The interlayer e-h exchange follows a similar process. The relative wave vector $\boldsymbol{q}_r$, $\boldsymbol{q}'_r$, and in-plane center-of-mass momentum $\boldsymbol{k}$ are denoted in the plot.

## S1. General description of the effective excitonic Hamiltonian in chiral bilayer systems

As previously stated in the main text, the construction of this Hamiltonian relies on two types of interaction: the electron-hole (e-h) exchange interaction between intralayer excitons of the same or different valleys in the same layer and the Förster coupling that

* wangyao@hku.hk

connects excitons in different layers, as illustrated in Fig. S1. The former interaction has been extensively studied in monolayer TMDs [1–3], and approximate expressions can be obtained by calculating the Coulomb exchange interaction between excitons in the same or different valleys [1, 2], or by solving the Bethe-Salpeter equation for e-h pair excitations [3]. Our derivation is based on the former approach [4]. For a specific layer $l$ ($l = t, b$ in this paper, $t/b$ means top/bottom layer, as shown in Fig. S1(a)) with at least two inequivalent valleys, $\boldsymbol{\alpha}$ and $\boldsymbol{\beta}$, one can define the creation operator for a bright exciton with the in-plane two-dimensional (2D) center-of-mass (COM) momentum $\boldsymbol{k} = (k\cos\varphi, k\sin\varphi)$ and twisted angle $\theta_l$ (relative to the untwisted layer):

$$\hat{B}^{\dagger}_{\boldsymbol{k},\alpha}(l) \equiv \sum_{\boldsymbol{q}_r} \psi\left(\mathcal{R}_{\theta_l}\boldsymbol{q}_r\right) \times \hat{e}^{\dagger}_{\mathcal{R}_{\theta_l}(\boldsymbol{\alpha}+\boldsymbol{q}_r)+\boldsymbol{k}^l_e,\uparrow} \hat{h}^{\dagger}_{\mathcal{R}_{\theta_l}(-\boldsymbol{\alpha}-\boldsymbol{q}_r)+\boldsymbol{k}^l_h,\Downarrow},$$
$$\hat{B}^{\dagger}_{\boldsymbol{k},\beta}(l) \equiv \sum_{\boldsymbol{q}_r} \psi\left(\mathcal{R}_{\theta_l}\boldsymbol{q}_r\right) \times \hat{e}^{\dagger}_{\mathcal{R}_{\theta_l}(\boldsymbol{\beta}+\boldsymbol{q}_r)+\boldsymbol{k}^l_e,\downarrow} \hat{h}^{\dagger}_{\mathcal{R}_{\theta_l}(-\boldsymbol{\beta}-\boldsymbol{q}_r)+\boldsymbol{k}^l_h,\Uparrow},$$
$$\boldsymbol{k}^l_{e/h} = \frac{m^{x,l}_{e/h,\lambda}}{m^{x,l}_{ex,\lambda}} k_x \hat{e}_x + \frac{m^{y,l}_{e/h,\lambda}}{m^{y,l}_{ex,\lambda}} k_y \hat{e}_y,$$

with $m^{\gamma,l}_{ex,\lambda}, \gamma = x, y$ is the exciton mass in $l$ layer for $\lambda$ valley, which can be expressed as

$$m^{\gamma,l}_{ex,\lambda} = m^{\gamma,l}_{e,\lambda} + m^{\gamma,l}_{h,\lambda},$$

i.e., the sum of effective electron and hole masses of the single-particle two-band $\boldsymbol{k}\cdot\boldsymbol{p}$ Hamiltonian. $\lambda = \alpha, \beta$ is the valley index. $\mathcal{R}_{\theta_l}\boldsymbol{q}_r$ $[\psi\left(\mathcal{R}_{\theta_l}\boldsymbol{q}_r\right)]$ is the relative wave vector [the wave function for the relative motion] between the electron and hole. Due to the twisted homobilayer structure we considered, the only difference between different layers is the twisted angle $\theta_l$. The $l$ index has been dropped in $\psi\left(\mathcal{R}_{\theta_l}\boldsymbol{q}_r\right)$ for simplicity since $\sum_{\boldsymbol{q}_r}\psi(\mathcal{R}_{\theta_l}\boldsymbol{q}_r) \approx \sum_{\boldsymbol{q}_r}\psi(\boldsymbol{q}_r)$. The hole operator in the valence band is defined as $\hat{h}^{\dagger}_{\boldsymbol{k},\Downarrow(\Uparrow)} \equiv \hat{e}^{\dagger}_{v,-\boldsymbol{k},\uparrow(\downarrow)}$, and the electron operator in the conduction band $\hat{e}^{\dagger}_{\boldsymbol{k},\uparrow(\downarrow)} \equiv \hat{e}^{\dagger}_{c,\boldsymbol{k},\uparrow(\downarrow)}$. $\uparrow, \downarrow$ is the spin index, which can be ignored for spinless or single-valley systems.

$$\mathcal{R}_{\theta_l} \equiv \begin{pmatrix} \cos\theta_l & -\sin\theta_l \\ \sin\theta_l & \cos\theta_l \end{pmatrix},$$

is a rotational operator in momentum space. $\mathcal{R}_{\theta_l}\boldsymbol{Q}$ means twisting the momentum $\boldsymbol{Q}$ for angle $\theta_l$ in the counterclockwise direction, which comes from the rotational operation $\mathcal{R}^{-1}_{\theta_l}\boldsymbol{r} = \mathcal{R}_{-\theta_l}\boldsymbol{r}$ in real space. According to this definition, the basis of valley excitons can be expressed

as

$$|l,\boldsymbol{k}\rangle_{\alpha}\equiv\hat{B}^{\dagger}_{\boldsymbol{k},\alpha}\left(l\right)|0\rangle\,,|l,\boldsymbol{k}\rangle_{\beta}\equiv\hat{B}^{\dagger}_{\boldsymbol{k},\beta}\left(l\right)|0\rangle\,, \tag{1}$$

$|0\rangle$ is the vacuum state for intralayer excitons and

$$\begin{pmatrix}\langle l,\boldsymbol{k}|_{\alpha}\\ \langle l,\boldsymbol{k}|_{\beta}\end{pmatrix}H^{l}_{\text{intra}}\left(|l,\boldsymbol{k}\rangle_{\alpha},|l,\boldsymbol{k}\rangle_{\beta}\right)$$
$$\equiv\begin{pmatrix}J^{l}_{\alpha,\alpha} & J^{l}_{\alpha,\beta}\\ J^{l}_{\beta,\alpha} & J^{l}_{\beta,\beta}\end{pmatrix}, \tag{2}$$

In detail [1, 2], the e-h intra- or intervalley exchange is

$$J^{l}_{\lambda,\lambda'}=\sum_{\boldsymbol{q}_r\boldsymbol{q}'_r}\psi\left(\mathcal{R}_{\theta_l}\boldsymbol{q}'_r\right)\psi^{*}\left(\mathcal{R}_{\theta_l}\boldsymbol{q}_r\right)J^{l}_{\lambda,\lambda'}\left(\mathcal{R}_{\theta_l}\boldsymbol{q}'_r,\mathcal{R}_{\theta_l}\boldsymbol{q}_r,\boldsymbol{k}\right), \tag{3}$$

$$\begin{aligned}&J^{l}_{\lambda,\lambda'}\left(\mathcal{R}_{\theta_l}\boldsymbol{q}'_r,\mathcal{R}_{\theta_l}\boldsymbol{q}_r,\boldsymbol{k}\right)\\ =&\sum_{\boldsymbol{G}}\frac{V\left(\boldsymbol{G}+\boldsymbol{k}\right)}{A}\times\\ &\left\langle u_{\mathcal{R}_{\theta_l}(\boldsymbol{\lambda}+\boldsymbol{q}_r)+\boldsymbol{k}^{l}_{e},c,S_{\alpha}}\right|e^{i\boldsymbol{G}\cdot\boldsymbol{r}}\left|u_{\mathcal{R}_{\theta_l}(\boldsymbol{\lambda}+\boldsymbol{q}_r)-\boldsymbol{k}^{l}_{h},v,S_{\alpha}}\right\rangle\times\\ &\left\langle u_{\mathcal{R}_{\theta_l}(\boldsymbol{\lambda}'+\boldsymbol{q}'_r)-\boldsymbol{k}^{l}_{h},v,S_{\beta}}\right|e^{-i\boldsymbol{G}\cdot\boldsymbol{r}}\left|u_{\mathcal{R}_{\theta_l}(\boldsymbol{\lambda}'+\boldsymbol{q}'_r)+\boldsymbol{k}^{l}_{e},c,S_{\beta}}\right\rangle,\end{aligned}$$

with $\lambda,\lambda'=\alpha,\beta$ and $S_{\alpha,\beta}=\uparrow,\downarrow$, as shown in Fig. S1(b). $\boldsymbol{G}$ is the reciprocal lattice vector for the untwisted layer ($\theta_l=0$), $A$ is the area of 2D plane. $\phi_{\boldsymbol{Q},c/v,\uparrow/\downarrow}\left(\boldsymbol{r}\right)=e^{i\boldsymbol{Q}\cdot\boldsymbol{r}}u_{\boldsymbol{Q},c/v,\uparrow/\downarrow}\left(\boldsymbol{r}\right)$ represents the Bloch wave function at the momentum $\boldsymbol{Q}$, and $V\left(\boldsymbol{Q}\right)=\int V\left(\boldsymbol{r}\right)e^{i\boldsymbol{Q}\cdot\boldsymbol{r}}d\,\boldsymbol{r}=2\pi e^{2}/\left(\epsilon Q\right)$ denotes the Coulomb potential in momentum space, which is the unscreened form of Coulomb interaction with $\epsilon\equiv4\pi\epsilon_0\epsilon_r$. Here only the long range part with $\boldsymbol{G}=0$ is vaild, since it has been shown that the short range part with $\boldsymbol{G}\neq0$ can be negligible in our consideration [4]. Using the $\boldsymbol{k}\cdot\boldsymbol{p}$ expansion to expand $\left|u_{\mathcal{R}_{\theta_l}(\boldsymbol{\lambda}+\boldsymbol{q}_r)\pm\boldsymbol{k}^{l}_{e/h},s=c,v}\right\rangle$ in the first order of $k$, it gives

$$\begin{aligned}&\left|u_{\mathcal{R}_{\theta_l}(\boldsymbol{\lambda}+\boldsymbol{q}_r)\pm\boldsymbol{k}^{l}_{e/h},s}\right\rangle\\ =&\left|u_{\mathcal{R}_{\theta_l}(\boldsymbol{\lambda}+\boldsymbol{q}_r),s}\right\rangle\mp\\ &\boldsymbol{k}^{l}_{e/h}\cdot\sum_{s'\neq s}\boldsymbol{d}_{s's,\mathcal{R}_{\theta_l}(\boldsymbol{\lambda}+\boldsymbol{q}_r)}\left|u_{\mathcal{R}_{\theta_l}(\boldsymbol{\lambda}+\boldsymbol{q}_r),s'}\right\rangle+O\left(k_{\parallel}^{2}\right),\end{aligned} \tag{4}$$

where we have omitted the spin index in here and the rest of the Supplementary for simplicity. $\boldsymbol{d}_{s's,\boldsymbol{Q}}=\frac{\hbar}{m_e}\frac{\langle u_{s',\boldsymbol{Q}}|\boldsymbol{p}|u_{s,\boldsymbol{Q}}\rangle}{\varepsilon_{s'}-\varepsilon_{s}}=-\boldsymbol{d}^{*}_{ss',\boldsymbol{Q}}$, $\boldsymbol{p}=-i\hbar\nabla$, $s's=cv$ or $vc$ is the optical transition dipole

between conduction ($c$) band and valence ($v$) band in the effective single-particle two-band $\boldsymbol{k}\cdot\boldsymbol{p}$ model near the valley, $m_e$ is the free electron mass, and $\varepsilon_{s=c,v}$ corresponds to the dispersion of $c$ or $v$ band respectively. As we showed in Fig. S2(a), the relation between the optical transition dipole in the untwisted layer, and twisted layer $l$ with the twisted angle $\theta_l$ can be expressed as

$$d^{x_l}_{s's,\mathcal{R}_{\theta_l}\boldsymbol{Q}} = d^{x}_{s's,\boldsymbol{Q}}, d^{y_l}_{s's,\mathcal{R}_{\theta_l}\boldsymbol{Q}} = d^{y}_{s's,\boldsymbol{Q}}.$$

So

$$\boldsymbol{d}_{s's,\mathcal{R}_{\theta_l}(\boldsymbol{\lambda}+\boldsymbol{q}_r)} = \mathcal{R}_{\theta_l}\boldsymbol{d}_{s's,\boldsymbol{\lambda}+\boldsymbol{q}_r}, \tag{5}$$

in the original untwisted Cartesian coordinate, which gives

$$\begin{aligned}
\left\langle u_{\mathcal{R}_{\theta_l}(\boldsymbol{\lambda}'+\boldsymbol{q}'_r)-\boldsymbol{k}^l_h,v}\middle| u_{\mathcal{R}_{\theta_l}(\boldsymbol{\lambda}'+\boldsymbol{q}'_r)+\boldsymbol{k}^l_e,c}\right\rangle \approx & -\left(\frac{k^l_{e,+}}{2}e^{-i\theta_l}d^-_{vc,\boldsymbol{\lambda}'+\boldsymbol{q}'_r}+\frac{k^l_{e,-}}{2}e^{i\theta_l}d^+_{vc,\boldsymbol{\lambda}'+\boldsymbol{q}'_r}\right)\\
&+\left(\frac{k^l_{h,+}}{2}e^{-i\theta_l}d^-_{cv,\boldsymbol{\lambda}'+\boldsymbol{q}'_r}+\frac{k^l_{h,-}}{2}e^{i\theta_l}d^+_{cv,\boldsymbol{\lambda}'+\boldsymbol{q}'_r}\right)^*\\
&=\left(\frac{k^l_{e,+}+k^l_{h,+}}{2}e^{-i\theta_l}d^-_{cv,\boldsymbol{\lambda}'+\boldsymbol{q}'_r}+\frac{k^l_{e,-}+k^l_{h,-}}{2}e^{i\theta_l}d^+_{cv,\boldsymbol{\lambda}'+\boldsymbol{q}'_r}\right)^*\\
&=\frac{1}{2}\left(k_+e^{-i\theta_l}d^-_{cv,\boldsymbol{\lambda}'+\boldsymbol{q}'_r}+k_-e^{i\theta_l}d^+_{cv,\boldsymbol{\lambda}'+\boldsymbol{q}'_r}\right)^*,
\end{aligned}$$

$$\begin{aligned}
\left\langle u_{\mathcal{R}_{\theta_l}(\boldsymbol{\lambda}+\boldsymbol{q}_r)+\boldsymbol{k}^l_e,c}\middle| u_{\mathcal{R}_{\theta_l}(\boldsymbol{\lambda}+\boldsymbol{q}_r)-\boldsymbol{k}^l_h,v}\right\rangle \approx & \left(\frac{k^l_{h,+}}{2}e^{-i\theta_l}d^-_{cv,\boldsymbol{\lambda}+\boldsymbol{q}_r}+\frac{k^l_{h,-}}{2}e^{i\theta_l}d^+_{cv,\boldsymbol{\lambda}+\boldsymbol{q}_r}\right)\\
&-\left(\frac{k^l_{e,+}}{2}e^{-i\theta_l}d^-_{vc,\boldsymbol{\lambda}+\boldsymbol{q}_r}+\frac{k^l_{e,-}}{2}e^{i\theta_l}d^+_{vc,\boldsymbol{\lambda}+\boldsymbol{q}_r}\right)^*\\
&=\frac{1}{2}\left(k_+e^{-i\theta_l}d^-_{cv,\boldsymbol{\lambda}'+\boldsymbol{q}'_r}+k_-e^{i\theta_l}d^+_{cv,\boldsymbol{\lambda}'+\boldsymbol{q}'_r}\right),
\end{aligned}$$

and

$$\begin{aligned}
J^l_{\lambda,\lambda'}(\boldsymbol{G}=0) \approx & \left[\psi^l_\lambda(\boldsymbol{r}_{eh}=0)\right]^*\psi^l_{\lambda'}(\boldsymbol{r}_{eh}=0)\frac{V(\boldsymbol{k})}{4}\times\\
&\left(k_+e^{-i\theta_l}d^-_{cv,\lambda}+k_-e^{i\theta_l}d^+_{cv,\lambda}\right)\times\\
&\left(k_+e^{-i\theta_l}d^-_{cv,\lambda'}+k_-e^{i\theta_l}d^+_{cv,\lambda'}\right)^*,
\end{aligned}\tag{6}$$

with $k_\pm = k_x \pm ik_y$, $d^\pm_{cv,\lambda} = d^x_{cv,\lambda} \pm id^y_{cv,\lambda}$. $\psi(\boldsymbol{r}_{eh}) = \frac{1}{\sqrt{A}}\sum_{\boldsymbol{q}_r}\psi(\mathcal{R}_{\theta_l}\boldsymbol{q}_r)e^{-i\mathcal{R}_{\theta_l}\boldsymbol{q}_r\cdot\boldsymbol{r}_{eh}}$ is the real space wavefunction for the relative motion between electron and hole, which comes from solving the Schrodinger equation of the hydrogen-like atom [5]. $\psi^l_\lambda(\boldsymbol{r}_{eh}=0) \equiv \psi^l_\lambda(0) \sim 1/\sqrt{a^{x,l}_{B,\lambda}a^{y,l}_{B,\lambda}}$ with the exciton Bohr radius $a^{\gamma,l}_{B,\lambda}, \gamma = x, y$ for $\lambda$ valley can be seen as the

square root of the probability for electron and hole to overlap in an exciton, and $d^{\gamma}_{cv,\lambda}$ according to the single-particle two-band $\boldsymbol{k}\cdot\boldsymbol{p}$ Hamiltonian [6].

From the same starting point, we can get the specific from of the Förster coupling between layer $l$ and $l'$ by using the same basis $\left\{|l,\boldsymbol{k}\rangle_{\alpha},|l,\boldsymbol{k}\rangle_{\beta}\right\}$

$$\begin{pmatrix} \langle l,\boldsymbol{k}|_{\alpha} \\ \langle l,\boldsymbol{k}|_{\beta} \end{pmatrix} H^{l,l'}_{\text{inter}} \left(|l',\boldsymbol{k}\rangle_{\alpha},|l',\boldsymbol{k}\rangle_{\beta}\right) \equiv \begin{pmatrix} J^{l,l'}_{\alpha,\alpha} & J^{l,l'}_{\alpha,\beta} \\ J^{l,l'}_{\beta,\alpha} & J^{l,l'}_{\beta,\beta} \end{pmatrix}. \tag{7}$$

As we shows in Fig. S1(b),

$$J^{l,l'}_{\lambda,\lambda'} = \sum_{\boldsymbol{q}_r\boldsymbol{q}'_r} \psi\left(\mathcal{R}_{\theta_{l'}}\boldsymbol{q}'_r\right)\psi^{*}\left(\mathcal{R}_{\theta_l}\boldsymbol{q}_r\right) J^{l,l'}_{\lambda,\lambda'}\left(\mathcal{R}_{\theta_{l'}}\boldsymbol{q}'_r,\mathcal{R}_{\theta_l}\boldsymbol{q}_r,\boldsymbol{k}\right), \tag{8}$$

$$\begin{aligned} & J^{l,l'}_{\lambda,\lambda'}\left(\mathcal{R}_{\theta_{l'}}\boldsymbol{q}'_r,\mathcal{R}_{\theta_l}\boldsymbol{q}_r,\boldsymbol{k}\right) \\ = & \sum_{\boldsymbol{G}} \frac{V\left(\boldsymbol{G}+\boldsymbol{k},\Delta z\right)}{A} \times \\ & \left\langle u_{\mathcal{R}_{\theta_l}(\boldsymbol{\lambda}+\boldsymbol{q}_r)+\boldsymbol{k}^l_e,c}\right| e^{i\boldsymbol{G}\cdot\boldsymbol{r}} \left| u_{\mathcal{R}_{\theta_l}(\boldsymbol{\lambda}+\boldsymbol{q}_r)-\boldsymbol{k}^l_h,v}\right\rangle \times \\ & \left\langle u_{\mathcal{R}_{\theta_{l'}}(\boldsymbol{\lambda}'+\boldsymbol{q}'_r)-\boldsymbol{k}^l_h,v}\right| e^{-i\boldsymbol{G}\cdot\boldsymbol{r}} \left| u_{\mathcal{R}_{\theta_{l'}}(\boldsymbol{\lambda}'+\boldsymbol{q}'_r)+\boldsymbol{k}^l_e,c}\right\rangle, \end{aligned}$$

where $V\left(\boldsymbol{Q},\Delta z\right) = \int V\left(\boldsymbol{r},\Delta z\right)e^{i\boldsymbol{Q}\cdot\boldsymbol{r}}d\boldsymbol{r} = 2\pi e^2/\left(\epsilon Q\right)\times\exp\left(-Q\Delta z\right)$. The extra exponential factor comes from the dependence of out-of-plane displacement $\Delta z$ between two layers for $V\left(\boldsymbol{r},\Delta z\right)$ [4]. This is a characteristic form of the Coulomb interaction in 2D momentum space [8–10], which can be seen as a good approximation for the broadly-used Rytova-Keldysh form in TMD heterostructure calculations [11–13] when the momentum $\boldsymbol{k}$ is sufficiently small. In this case, $\epsilon$ can be interpreted as an effective dielectric constant if the surrounding dielectric medium is anisotropic [13]. The short range part of this coupling is still ignorable and the long range part leads to

$$\begin{aligned} J^{l,l'}_{\lambda,\lambda'} \approx & \left[\psi^{l}_{\lambda}(0)\right]^{*}\psi^{l'}_{\lambda'}(0)\frac{V\left(\boldsymbol{k},\Delta z\right)}{4}\times \\ & \left(k_{+}e^{-i\theta_l}d^{-}_{cv,\lambda}+k_{-}e^{i\theta_l}d^{+}_{cv,\lambda}\right)\times \\ & \left(k_{+}e^{-i\theta_{l'}}d^{-}_{cv,\lambda'}+k_{-}e^{i\theta_{l'}}d^{+}_{cv,\lambda'}\right)^{*}, \end{aligned} \tag{9}$$

where we take $\Delta z = 1\,\text{nm}$ in the main text as a typical value.

At last, every valley exciton in each layer has its own kinetic energy, which brings the kinetic energy term as

$$H_k^l = \begin{pmatrix} \frac{\hbar^2 k_x^2}{2m_{ex,\alpha}^{x,l}} + \frac{\hbar^2 k_y^2}{2m_{ex,\alpha}^{y,l}} & 0 \\ 0 & \frac{\hbar^2 k_x^2}{2m_{ex,\beta}^{x,l}} + \frac{\hbar^2 k_y^2}{2m_{ex,\beta}^{y,l}} \end{pmatrix}, \tag{10}$$

Since there is a twist angle $\theta_l$ for $l$ layer, the $xy$ coordinate $(\hat{x}, \hat{y})$ in the untwisted layer can be connected with $(\hat{x}_l, \hat{y}_l)$ by the rotational matrix $\mathcal{R}_{\theta_l}$

$$\begin{pmatrix} \hat{x}_l \\ \hat{y}_l \end{pmatrix} = \begin{pmatrix} \cos\theta_l & -\sin\theta_l \\ \sin\theta_l & \cos\theta_l \end{pmatrix} \begin{pmatrix} \hat{x} \\ \hat{y} \end{pmatrix},$$

as shown in Fig. S2(a). According to

$$\frac{\hbar^2}{2m_{e,\lambda}^{\gamma,l}} = \frac{\partial^2 \varepsilon_{c,\lambda}^l}{\partial q_\gamma^2}, \frac{\hbar^2}{2m_{h,\lambda}^{\gamma,l}} = -\frac{\partial^2 \varepsilon_{v,\lambda}^l}{\partial q_\gamma^2},$$

with $\varepsilon_{s,\lambda}^l$ corresponds to the dispersion of $c$ or $v$ band near $\lambda$ valley in $l$ layer. One can easily find that

$$\begin{aligned} \frac{\partial^2 \varepsilon_{s,\lambda}^l}{\partial q_\gamma^2} &= \frac{\partial}{\partial q_\gamma} \frac{\partial \varepsilon_{s,\lambda}^l}{\partial q_\gamma} \\ &= \frac{\partial}{\partial q_\gamma} \left( \frac{\partial q_{x_l}}{\partial q_\gamma} \frac{\partial \varepsilon_{s,\lambda}^l}{\partial q_{x_l}} + \frac{\partial q_{y_l}}{\partial q_\gamma} \frac{\partial \varepsilon_{s,\lambda}^l}{\partial q_{y_l}} \right) \\ &= \left( \frac{\partial q_{x_l}}{\partial q_\gamma} \frac{\partial}{\partial q_{x_l}} + \frac{\partial q_{y_l}}{\partial q_\gamma} \frac{\partial}{\partial q_{y_l}} \right) \left( \frac{\partial \varepsilon_{s,\lambda}^l}{\partial q_{x_l}} \frac{\partial q_{x_l}}{\partial q_\gamma} + \frac{\partial \varepsilon_{s,\lambda}^l}{\partial q_{y_l}} \frac{\partial q_{y_l}}{\partial q_\gamma} \right) \\ &\approx \frac{\partial^2 \varepsilon_{s,\lambda}^l}{\partial q_{x_l}^2} \left( \frac{\partial q_{x_l}}{\partial q_\gamma} \right)^2 + \frac{\partial^2 \varepsilon_{s,\lambda}^l}{\partial q_{y_l}^2} \left( \frac{\partial q_{y_l}}{\partial q_\gamma} \right)^2, \end{aligned}$$

where terms including $\frac{\partial^2 \varepsilon_{s,\lambda}^l}{\partial q_{x_l} \partial q_{y_l}}$ have been vanished due to $\varepsilon_{s,\lambda}^l \approx \frac{\hbar^2 q_{x_l}^2}{2m_{s,\lambda}^x} + \frac{\hbar^2 q_{y_l}^2}{2m_{s,\lambda}^x}$ in the single-particle two-band $\boldsymbol{k} \cdot \boldsymbol{p}$ Hamiltonian. Above derivation leads to

$$\begin{aligned} \frac{\hbar^2}{2m_{s,\lambda}^{x,l}} &= \frac{\partial^2 \varepsilon_{s,\lambda}^l}{\partial q_x^2} = \frac{\hbar^2}{2m_{s,\lambda}^x} \cos^2\theta_l + \frac{\hbar^2}{2m_{s,\lambda}^y} \sin^2\theta_l, \\ \frac{\hbar^2}{2m_{s,\lambda}^{y,l}} &= \frac{\partial^2 \varepsilon_{s,\lambda}^l}{\partial q_y^2} = \frac{\hbar^2}{2m_{s,\lambda}^x} \sin^2\theta_l + \frac{\hbar^2}{2m_{s,\lambda}^y} \cos^2\theta_l, \end{aligned}$$

and

$$m_{s,\lambda}^{x,l} = \frac{m_{s,\lambda}^x m_{s,\lambda}^y}{m_{s,\lambda}^y \cos^2\theta_l + m_{s,\lambda}^x \sin^2\theta_l}, m_{s,\lambda}^{y,l} = \frac{m_{s,\lambda}^x m_{s,\lambda}^y}{m_{s,\lambda}^y \sin^2\theta_l + m_{s,\lambda}^x \cos^2\theta_l}, \tag{11}$$

i.e., $m_{ex,\lambda}^{\gamma,l}$ is dependent on the twisted angle $\theta_l$. Moreover, one should attention that the exciton Bohr radius $a_{B,\lambda}^{\gamma,l}$ can be approximately represented in the form

$$a_{B,\lambda}^{\gamma,l} \approx \frac{\epsilon_r}{\mu_\lambda^{\gamma,l}/m_e} a_0,$$

$a_0 \approx 0.53\,\text{Å}$ is Bohr radius constant. Since the reduced mass of the e-h pair $\mu_\lambda^{\gamma,l}$ for $\lambda$ valley in $l$ layer is defined as

$$\mu_\lambda^{\gamma,l} = \frac{m_{e,\lambda}^{\gamma,l} m_{h,\lambda}^{\gamma,l}}{m_{e,\lambda}^{\gamma,l} + m_{h,\lambda}^{\gamma,l}},$$

it means $a_{B,\lambda}^{\gamma,l}$ is also dependent on $\theta_l$, as well as $\psi_\lambda^l(0)$.

### A. Excitonic Hamiltonian of TMDs

Without loss of generality, let $\theta_b = 0$, $\theta_t = \theta$ and replace the twist angle $\theta$ in momentum space into the real space one, i.e., $\theta \to -\theta$ in the rest of the Supplementary. Since the single-particle two-band $\boldsymbol{k}\cdot\boldsymbol{p}$ Hamiltonian for each valley ($\alpha, \beta = \pm K$) in TMDs is the Dirac model [6], the isotropic feature leads to $\psi_\lambda^l(0) \sim \psi(0) \sim 1/a_B$ with $a_B \approx 1\,\text{nm}$ [2, 5, 14], and

$$H_k^l = H_k = \frac{\hbar^2 k^2}{2m_{ex}}.$$

Then the effective Hamiltonian of valley excitons in the twisted homobilayer TMD can be written as

$$H_{\text{TMD}} = \frac{\hbar^2 k^2}{2m_{ex}} + \sum_{l=t,b} H_{\text{intra}}^l + \sum_{l,l'=t,b} H_{\text{inter}}^{l,l'}, \tag{12}$$

in the basis $\left\{ |l,\boldsymbol{k}\rangle_K, |l,\boldsymbol{k}\rangle_{-K} \right\}$, with

$$H_{\text{intra}}^b = J\frac{k}{K}\begin{pmatrix} 1 & -e^{-2i\varphi} \\ -e^{2i\varphi} & 1 \end{pmatrix},$$

$$H_{\text{intra}}^t = J\frac{k}{K}\begin{pmatrix} 1 & -e^{-2i(\theta+\varphi)} \\ -e^{2i(\theta+\varphi)} & 1 \end{pmatrix},$$

and

$$H_{\text{inter}}^{b,t} = \left(H_{\text{inter}}^{t,b}\right)^\dagger = J\frac{k}{K}e^{-k\Delta z}\begin{pmatrix} e^{i\theta} & -e^{-i(\theta+2\varphi)} \\ -e^{i(\theta+2\varphi)} & e^{-i\theta} \end{pmatrix}.$$

$m_{ex} \approx m_e$ is the effective exciton mass in monolayer TMDs. By using the parameters of monolayer $WSe_2$ [2, 6], $K \equiv 4\pi/3a = 1.26\,\text{Å}^{-1}$ is the distance from $K$ to $\Gamma$ point, which

gives the size of the Brillouin zone. $J \approx 1\,\mathrm{eV}$ comes from the first-principle calculation [4]. The Hamiltonian in Eq. (12) can be diagonalized from the eigen branches of $H^{l}_{\mathrm{intra}}$

$$\begin{aligned} |l,\boldsymbol{k}\rangle_{L} &= \frac{-e^{-i(\theta_l+2\varphi)}\,|l,\boldsymbol{k}\rangle_{K} + e^{i\theta_l}\,|l,\boldsymbol{k}\rangle_{-K}}{\sqrt{2}}, \\ |l,\boldsymbol{k}\rangle_{T} &= \frac{e^{-i\theta_l}\,|l,\boldsymbol{k}\rangle_{K} + e^{i(2\varphi+\theta_l)}\,|l,\boldsymbol{k}\rangle_{-K}}{\sqrt{2}}, \end{aligned} \tag{13}$$

leading to

$$H_{\mathrm{TMD}} = \begin{pmatrix} \varepsilon_L & 2J\frac{k}{K}e^{-k\Delta z} & 0 & 0 \\ 2J\frac{k}{K}e^{-k\Delta z} & \varepsilon_L & 0 & 0 \\ 0 & 0 & \varepsilon_T & 0 \\ 0 & 0 & 0 & \varepsilon_T \end{pmatrix}, \tag{14}$$

with $\varepsilon_L = \frac{\hbar^2 k^2}{2m_{ex}} + 2J\frac{k}{K}$ and $\varepsilon_T = \frac{\hbar^2 k^2}{2m_{ex}}$, which is independent of the twist angle $\theta$. The degenerate dispersion $\varepsilon_T$ is associated with $|l,\boldsymbol{k}\rangle_T$, while $\left(|b,\boldsymbol{k}\rangle_L \pm |t,\boldsymbol{k}\rangle_L\right)/\sqrt{2}$ correspond to $\varepsilon_L \pm 2J\frac{k}{K}e^{-k\Delta z}$, respectively.

Previous studies have proved that if there is a strain for the bottom layer (coming from the operation to the substrate) of the twisted bilayer structure, a strain transfer can happen between the bottom layer and the top one [15, 16]. The efficiency of this effect is significantly influenced by the twisted angle, where the small or aligned angle (60°) leads to nearly 100% strain transfer and the large or unaligned angle will reduce the transfer to 40~60%, respectively. This experimental data can be described by an approximate function as

$$\eta_\theta = \begin{cases} \frac{3}{4} + \frac{1}{4}\sin\pi\left(\frac{n\pi/3+7.5^\circ-\theta}{5}\right), \theta \in \left[\frac{n\pi}{3}+5^\circ, \frac{n\pi}{3}+10^\circ\right], \\ 0.5, \theta \in \left[\frac{n\pi}{3}+10^\circ, \frac{(n+1)\pi}{3}-10^\circ\right], \\ \frac{3}{4} - \frac{1}{4}\sin\pi\left(\frac{(n+1)\pi/3-7.5^\circ-\theta}{5}\right), \theta \in \left[\frac{(n+1)\pi}{3}-10^\circ, \frac{(n+1)\pi}{3}-5^\circ\right], \\ 1, \theta \in \left[\frac{n\pi}{3}-5^\circ, \frac{n\pi}{3}+5^\circ\right], \end{cases}, n \in [0,5], \tag{15}$$

as shown in Fig. S2(c). On the other hand, it has been found that large strain cannot be transfered between van der Waals layers [15], the efficiency would drop obviously if the strain is over 2%.

However, in most of cases considered by the earlier researches, the two layers contact directly without the spacer. Generally, the existence of the spacer between two layers is expected to reduce the influence from the physical modulation of the bottom layer to the top one. Based on this general understanding, we assume that the hBN spacer in our

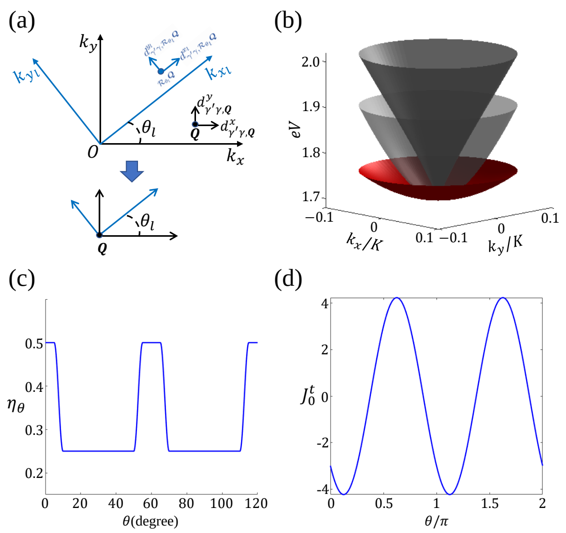

FIG. S2. (color online)(a) Schematic illustration of the relation between the optical transition dipole $\boldsymbol{d}_{s's,\boldsymbol{Q}}$ in the untwisted layer and twisted layer $l$. $\boldsymbol{Q}$ denotes the momentum near the $K$ or $-K$ valley. $s's = vc$ or $cv$ indicates the band index for conduction ($c$) and valence ($v$) bands. A similar relationship can be found between $xy$ coordinate $(\hat{x}, \hat{y})$ in the untwisted layer and $(\hat{x}_l, \hat{y}_l)$ in the twisted layer. (b) Excitonic bands of the effective Hamiltonian $H_{TMD}$ (Eq. 12). Two degenerate bands $\varepsilon_T$ are shown in red, while $\varepsilon_L \pm 2J\frac{k}{K}e^{-k\Delta z}$ are represented as gray and deeper gray, respectively. (c) $\eta_\theta$ in Eq. (15) as a function of the twisted angle $\theta$, which is periodic with a periodicity of $\pi/3$. (d) $J_0^t$ as a function of $\theta$ by setting $\eta_\theta \equiv 1$.

consideration can reduce the strain transfer as

$$\epsilon_{st,t}(\theta) = \eta_\theta \eta_{\text{int}} \epsilon_{st,b}, \tag{16}$$

with $\eta_{\text{int}} \approx 0.5$, where $\epsilon_{st,b/st,t}$ means the strain of the bottom/top layer, $\eta_{\theta/\text{int}}$ represents the efficiency of strain transfer with respect to twisted angle/spacer between two layers.

Normally, a strain in 2D real space can be expressed as [17–19]

$$\begin{aligned} \overleftrightarrow{\epsilon} = \begin{pmatrix} \epsilon_{xx} & \epsilon_{xy} \\ \epsilon_{yx} & \epsilon_{yy} \end{pmatrix} \begin{pmatrix} \hat{x} \\ \hat{y} \end{pmatrix} &= R^{-1}(\phi) \begin{pmatrix} \epsilon_{st} & 0 \\ 0 & -v\epsilon_{st} \end{pmatrix} R(\phi) \begin{pmatrix} \hat{x} \\ \hat{y} \end{pmatrix} \\ &= \begin{pmatrix} \cos\phi & \sin\phi \\ -\sin\phi & \cos\phi \end{pmatrix} \begin{pmatrix} \epsilon_{st} & 0 \\ 0 & -v\epsilon_{st} \end{pmatrix} \begin{pmatrix} \cos\phi & -\sin\phi \\ \sin\phi & \cos\phi \end{pmatrix} \begin{pmatrix} \hat{x} \\ \hat{y} \end{pmatrix} \\ &= \epsilon_{st} \begin{pmatrix} \cos^2\phi - v\sin^2\phi & -\frac{1+v}{2}\sin 2\phi \\ -\frac{1+v}{2}\sin 2\phi & \sin^2\phi - v\cos^2\phi \end{pmatrix} \begin{pmatrix} \hat{x} \\ \hat{y} \end{pmatrix}, \end{aligned} \tag{17}$$

where $v$ is Poisson ratio of the material (In TMDs, $v \approx 0.23$ [19]), the angle $\phi$ means the strain direction. So for any lattice vector $\boldsymbol{r}$ in 2D real space, we have $\boldsymbol{r} \rightarrow (1 + \overleftrightarrow{\epsilon})\,\boldsymbol{r}$, which means any reciprocal vector in 2D momentum space should be transformed into $\boldsymbol{G} \rightarrow (1 + \overleftrightarrow{\epsilon})^{-1}\,\boldsymbol{G}$ with

$$
\begin{aligned}
(1+\overleftrightarrow{\epsilon})^{-1} &= \left[1 + \epsilon_{st}\begin{pmatrix} \cos^2\phi - v\sin^2\phi & -\frac{1+v}{2}\sin 2\phi \\ -\frac{1+v}{2}\sin 2\phi & \sin^2\phi - v\cos^2\phi \end{pmatrix}\right]^{-1} \\
&= \frac{1}{|1+\overleftrightarrow{\epsilon}|}\left[1 + \epsilon_{st}\begin{pmatrix} \sin^2\phi - v\cos^2\phi & \frac{1+v}{2}\sin 2\phi \\ \frac{1+v}{2}\sin 2\phi & \cos^2\phi - v\sin^2\phi \end{pmatrix}\right], \\
|1+\overleftrightarrow{\epsilon}| &= 1 + \epsilon_{st}\,(1-v) - \epsilon_{st}^2 v\left(\cos^4\phi + \sin^4\phi\right).
\end{aligned}
\tag{18}
$$

Specially, for $\phi = 0$

$$
(1+\overleftrightarrow{\epsilon})^{-1} = \left[1 + \begin{pmatrix} \epsilon_{st} & 0 \\ 0 & -v\epsilon_{st} \end{pmatrix}\right]^{-1} = \begin{pmatrix} \frac{1}{1+\epsilon_{st}} & 0 \\ 0 & \frac{1}{1-v\epsilon_{st}} \end{pmatrix},
$$

for $\phi = \pi/2$

$$
(1+\overleftrightarrow{\epsilon})^{-1} = \left[1 + \begin{pmatrix} -v\epsilon_{st} & 0 \\ 0 & \epsilon_{st} \end{pmatrix}\right]^{-1} = \begin{pmatrix} \frac{1}{1-v\epsilon_{st}} & 0 \\ 0 & \frac{1}{1+\epsilon_{st}} \end{pmatrix}.
$$

According to these two conditions,

$$
\begin{aligned}
\boldsymbol{G}\cdot\boldsymbol{r} &\rightarrow \boldsymbol{G}\left[(1+\overleftrightarrow{\epsilon})^{-1}\right]^{T}\cdot(1+\overleftrightarrow{\epsilon})\,\boldsymbol{r} \\
&= \boldsymbol{G}\,(1+\overleftrightarrow{\epsilon})^{-1}\cdot(1+\overleftrightarrow{\epsilon})\,\boldsymbol{r} = \boldsymbol{G}\cdot\boldsymbol{r}.
\end{aligned}
\tag{19}
$$

For the high symmetry points which are located at the gap between conduction and valence bands, i.e., the valleys, the transition of the position in momentum space is a little different, which is

$$
\pm\boldsymbol{K} \rightarrow \pm\,(1+\overleftrightarrow{\epsilon})^{-1}\,\boldsymbol{K} - \boldsymbol{A}_s, \tag{20}
$$

where

$$
\begin{aligned}
\boldsymbol{A}_s &= \pm\beta\,|\boldsymbol{K}|\,(\epsilon_{xx} - \epsilon_{yy}, -2\epsilon_{xy})^{T} \\
&= \pm\epsilon_{st}\,(1+v)\,\beta\,|\boldsymbol{K}|\begin{pmatrix} \cos 2\phi \\ \sin 2\phi \end{pmatrix},
\end{aligned}
$$

is the pseudovector potential due to the strain modulation of the intralayer hopping, where time-reversal symmetry requires the opposite sign at $\boldsymbol{K}$ and $-\boldsymbol{K}$ valleys. $\beta$ is a material-dependent parameter [17, 19]. However, since the strain considered in the theoretical and

experimental situations is always in the order of 1%˜3%, i.e., $\epsilon_{st} \approx 0.01˜0.03$, the related change of position for high symmetry points are pretty small, leading to the eigenwavefunction $\left|u_{\pm\boldsymbol{K},v/c}\right\rangle$ of the approximate single-particle two-band model near those high symmetry points keeps unchanged, also the Bohr radius of the exciton.

Based on all these analysis, the short-range e-h Coulomb exchange interaction between two valleys in monolayer TMDs can be expressed as [2]

$$\begin{aligned} J_{\boldsymbol{k}=0}^{\mathrm{SR}} \approx & \sum_{\boldsymbol{G}\neq 0} \frac{V(\boldsymbol{G})}{A} \sum_{\boldsymbol{q}_r'} \left[\psi^*(\boldsymbol{q}_r') \langle u_{\pm\boldsymbol{K},c}| e^{i\boldsymbol{G}\cdot\boldsymbol{r}} |u_{\pm\boldsymbol{K},v}\rangle\right] \\ & \times \sum_{\boldsymbol{q}_r} \left[\psi(\boldsymbol{q}_r) \langle u_{\pm\boldsymbol{K},v}| e^{-i\boldsymbol{G}\cdot\boldsymbol{r}} |u_{\pm\boldsymbol{K},c}\rangle\right] \\ \approx & \left|\psi(\boldsymbol{r}_{eh}=0)\right|^2 \sum_{\boldsymbol{G}\neq 0} V(\boldsymbol{G}) \langle u_{\pm\boldsymbol{K},c}| e^{i\boldsymbol{G}\cdot\boldsymbol{r}} |u_{\pm\boldsymbol{K},v}\rangle \langle u_{\pm\boldsymbol{K},v}| e^{-i\boldsymbol{G}\cdot\boldsymbol{r}} |u_{\pm\boldsymbol{K},c}\rangle , \end{aligned} \tag{21}$$

with $\left|\psi(\boldsymbol{r}_{eh}=0)\right|^2 \sim 1/a_B^2, a_B \approx 1\,\mathrm{nm}$, $V(\boldsymbol{G}) = 2\pi e^2/(\epsilon G)$ due to the negligible screening effect suppressed by large $\boldsymbol{G}$. Here, the diagonal part $J_{K,K}^{\mathrm{SR}}\left(J_{-K,-K}^{\mathrm{SR}}\right)$ only contributes to an energy shift ($5 \sim 6\,\mathrm{meV}$) that can be absorbed into the binding energy of excitons [1]. The original zero non-diagonal part $J_{K,-K}^{\mathrm{SR}}\left(J_{-K,K}^{\mathrm{SR}}\right)$ is no longer zero now since the three fold rotational symmetry has been broken by the strain, giving

$$\begin{aligned} J_0 \equiv & \left|\psi(\boldsymbol{r}_{eh}=0)\right|^2 \sum_{\boldsymbol{G}\neq 0} V(\boldsymbol{G}) \langle u_{\boldsymbol{K},c}| e^{i\boldsymbol{G}\cdot\boldsymbol{r}} |u_{\boldsymbol{K},v}\rangle \langle u_{-\boldsymbol{K},v}| e^{-i\boldsymbol{G}\cdot\boldsymbol{r}} |u_{-\boldsymbol{K},c}\rangle \\ \approx & \frac{2\pi e^2}{\sqrt{3}\epsilon K} \frac{1}{a_B^2} \sum_{\boldsymbol{G}\neq 0} \frac{\sqrt{3}K}{G} \langle u_{\boldsymbol{K},c}| e^{i\boldsymbol{G}\cdot\boldsymbol{r}} |u_{\boldsymbol{K},v}\rangle \langle u_{-\boldsymbol{K},v}| e^{-i\boldsymbol{G}\cdot\boldsymbol{r}} |u_{-\boldsymbol{K},c}\rangle \\ = & \frac{2\pi e^2}{\sqrt{3}\epsilon K} \frac{1}{a_B^2} \times f_s. \end{aligned} \tag{22}$$

The earlier studies have shown that the specific values of $f_s$, which are from the first-principle calculation [2], in different extent of strain along $x$ or $y$ direction. The Poisson ratio $v$ in this consideration has been set to zero, also the change of positions of the high symmetry points ($\boldsymbol{A}_s$) in momentum space for simplicity. So if the strain is along $x$ direction

$$\boldsymbol{G} \to \boldsymbol{G}_x = \begin{pmatrix} \frac{1}{1+\epsilon_{st}} & 0 \\ 0 & 1 \end{pmatrix} \boldsymbol{G} = \begin{pmatrix} \frac{A_n}{1+\epsilon_{st}} \\ B_n \end{pmatrix},$$

the strain along $y$ direction gives

$$\boldsymbol{G} \to \boldsymbol{G}_y = \begin{pmatrix} 1 & 0 \\ 0 & \frac{1}{1+\epsilon_{st}} \end{pmatrix} \boldsymbol{G} = \begin{pmatrix} A_n \\ \frac{B_n}{1+\epsilon_{st}} \end{pmatrix},$$

with $\boldsymbol{G}=(A_n,B_n)^T$ and

$$\begin{aligned}\frac{1}{G_x}&=\frac{1}{|\boldsymbol{G}_x|} \\ &=\frac{1}{\sqrt{\frac{A_n^2}{(1+\epsilon_{st})^2}+B_n^2}}=\frac{1+\epsilon_{st}}{\sqrt{A_n^2+B_n^2+2\epsilon_{st}B_n^2+\epsilon_{st}^2B_n^2}} \\ &\approx\frac{1+\epsilon_{st}}{\sqrt{|G|^2+2\epsilon_{st}B_n^2}}\approx(1+\epsilon_{st})\left[\frac{1}{|G|}-\frac{B_n^2}{|G|^3}\epsilon_{st}\right] \\ &=\frac{1+\epsilon_{st}}{|G|}\left[1-\frac{B_n^2}{|G|^2}\epsilon_{st}\right].\end{aligned}\tag{23}$$

The similar process gives

$$\frac{1}{G_y}=\frac{1}{|\boldsymbol{G}_y|}\approx\frac{1+\epsilon_{st}}{|G|}\left[1-\frac{A_n^2}{|G|^2}\epsilon_{st}\right],$$

leading to

$$\frac{1}{G_x}+\frac{1}{G_y}\approx\frac{1+\epsilon_{st}}{|G|}\left(2-\epsilon_{st}\right).$$

Since $\epsilon_{st}=0$ results in $J^{\mathrm{SR}}_{\boldsymbol{k}=0}=0$, i.e., $\sum_{\boldsymbol{G}\neq 0}\frac{\sqrt{3}K}{G}\langle u_{\boldsymbol{K},c}|\,e^{i\boldsymbol{G}\cdot\boldsymbol{r}}\,|u_{\boldsymbol{K},v}\rangle\langle u_{-\boldsymbol{K},v}|\,e^{-i\boldsymbol{G}\cdot\boldsymbol{r}}\,|u_{-\boldsymbol{K},c}\rangle=0$ for $\epsilon_{st}=0$, we can simplify above expressions to

$$\frac{1}{G_x}\approx-\frac{1+\epsilon_{st}}{|G|^3}B_n^2\epsilon_{st},\ \frac{1}{G_y}\approx-\frac{1+\epsilon_{st}}{|G|^3}A_n^2\epsilon_{st},\tag{24}$$

in calculation of $J^{\mathrm{SR}}_{\boldsymbol{k}=0}$ due to only these parts make non-zero contributions. On the other hand

$$\begin{aligned}\boldsymbol{G}_\phi&=\frac{1}{1+\epsilon_{st}}\begin{pmatrix}1+\epsilon_{st}\sin^2\phi & \frac{\epsilon_{st}}{2}\sin 2\phi\\ \frac{\epsilon_{st}}{2}\sin 2\phi & 1+\epsilon_{st}\cos^2\phi\end{pmatrix}\boldsymbol{G} \\ &=\begin{pmatrix}\frac{1+\epsilon_{st}\sin^2\phi}{1+\epsilon_{st}}A_n+\frac{\epsilon_{st}}{2}\frac{\sin 2\phi}{1+\epsilon_{st}}B_n\\ \frac{\epsilon_{st}}{2}\frac{\sin 2\phi}{1+\epsilon_{st}}A_n+\frac{1+\epsilon_{st}\cos^2\phi}{1+\epsilon_{st}}B_n\end{pmatrix},\end{aligned}\tag{25}$$

giving

$$\begin{aligned}\frac{1}{G_\phi}&\approx\frac{1+\epsilon_{st}}{\sqrt{|G|^2+2\epsilon_{st}\left(A_n\sin\phi+B_n\cos\phi\right)^2}} \\ &\approx(1+\epsilon_{st})\left[\frac{1}{|G|}-\frac{\left(A_n\sin\phi+B_n\cos\phi\right)^2}{|G|^3}\epsilon_{st}\right] \\ &=-\frac{1+\epsilon_{st}}{|G|^3}\left(A_n\sin\phi+B_n\cos\phi\right)^2\epsilon_{st} \\ &=-\frac{1+\epsilon_{st}}{|G|^3}\left(A_n^2\sin^2\phi+B_n^2\cos^2\phi+A_nB_n\sin 2\phi\right)\epsilon_{st}.\end{aligned}$$

Therefore, for any specific $\boldsymbol{G}$

$$
\begin{aligned}
f_{s,x}^{n} &\approx \frac{\sqrt{3}K}{G_x} \langle u_{\boldsymbol{K},c}| e^{i\boldsymbol{G}\cdot\boldsymbol{r}} |u_{\boldsymbol{K},v}\rangle \langle u_{-\boldsymbol{K},v}| e^{-i\boldsymbol{G}\cdot\boldsymbol{r}} |u_{-\boldsymbol{K},c}\rangle = \frac{\sqrt{3}K}{G_x} f_n \\
&\approx -\sqrt{3}K \frac{1+\epsilon}{|G|^3} B_n^2 \epsilon_{st} f_n, \\
f_{s,y}^{n} &\approx \frac{\sqrt{3}K}{G_y} \langle u_{\boldsymbol{K},c}| e^{i\boldsymbol{G}\cdot\boldsymbol{r}} |u_{\boldsymbol{K},v}\rangle \langle u_{-\boldsymbol{K},v}| e^{-i\boldsymbol{G}\cdot\boldsymbol{r}} |u_{-\boldsymbol{K},c}\rangle \\
&\approx -\sqrt{3}K \frac{1+\epsilon}{|G|^3} A_n^2 \epsilon_{st} f_n,
\end{aligned}
\tag{26}
$$

$$
\begin{aligned}
f_{s,\phi}^{n} &\approx \frac{\sqrt{3}K}{G_\phi} \langle u_{\boldsymbol{K},c}| e^{i\boldsymbol{G}\cdot\boldsymbol{r}} |u_{\boldsymbol{K},v}\rangle \langle u_{-\boldsymbol{K},v}| e^{-i\boldsymbol{G}\cdot\boldsymbol{r}} |u_{-\boldsymbol{K},c}\rangle \\
&\approx -\sqrt{3}K \frac{1+\epsilon}{|G|^3} \left(A_n^2 \sin^2\phi + B_n^2 \cos^2\phi + A_n B_n \sin 2\phi\right) \epsilon_{st} f_n \\
&= f_{s,x}^{n} \cos^2\phi + f_{s,y}^{n} \sin^2\phi - \sqrt{f_{s,x}^{n} f_{s,y}^{n}} \sin 2\phi.
\end{aligned}
$$

Then for the sum of non-zero $G$

$$
\begin{aligned}
f_{s,x} &\approx \sum_{\boldsymbol{G}\neq 0} f_{s,x}^{n} = \sum_{\boldsymbol{G}\neq 0} \frac{\sqrt{3}K}{G_x} f_n \approx -\sum_{\boldsymbol{G}\neq 0} \sqrt{3}K \frac{1+\epsilon_{st}}{|G|^3} B_n^2 \epsilon_{st} f_n, \\
f_{s,y} &\approx \sum_{\boldsymbol{G}\neq 0} f_{s,y}^{n} \approx -\sum_{\boldsymbol{G}\neq 0} \sqrt{3}K \frac{1+\epsilon_{st}}{|G|^3} A_n^2 \epsilon_{st} f_n,
\end{aligned}
$$

with $f_{s,x} + f_{s,y} \approx 0$.

$$
\begin{aligned}
f_{s,\phi} &\approx \sum_{\boldsymbol{G}\neq 0} f_{s,\phi}^{n} \\
&\approx -\sum_{\boldsymbol{G}\neq 0} \sqrt{3}K \frac{1+\epsilon_{st}}{|G|^3} \left(A_n^2 \sin^2\phi + B_n^2 \cos^2\phi + A_n B_n \sin 2\phi\right) \epsilon_{st} f_n.
\end{aligned}
$$

Here we roughly have

$$
-\sum_{\boldsymbol{G}\neq 0} \sqrt{3}K \frac{1+\epsilon}{|G|^3} A_n B_n \epsilon_{st} f_n \approx f_{s,x} \approx -f_{s,y}, \tag{27}
$$

and

$$
\begin{aligned}
f_{s,\phi} &\approx f_{s,x} \cos^2\phi + f_{s,y} \sin^2\phi + f_{s,x} \sin 2\phi \\
&= f_{s,x} \left(\cos 2\phi + \sin 2\phi\right).
\end{aligned}
\tag{28}
$$

According to above information, the new effective excitonic Hamiltonian of twisted bilayer TMDs, which includes the short-range e-h exchange interaction, can be expressed as

$$
H = H_{\mathrm{TMD}} = \frac{\hbar^2 k^2}{2m_{ex}} + \sum_{l=t,b} H_{\mathrm{intra}}^{l} + \sum_{l,l'=t,b} H_{\mathrm{inter}}^{l,l'}, \tag{29}
$$

still in the basis $\left\{|l,\boldsymbol{k}\rangle_K, |l,\boldsymbol{k}\rangle_{-K}\right\}$, with

$$H^l_{\text{intra}} = \begin{pmatrix} J\frac{k_\parallel}{K} & J^l_0 - J\frac{k_\parallel}{K}e^{-2i(\theta_l+\varphi)} \\ J^l_0 - J\frac{k_\parallel}{K}e^{2i(\theta_l+\varphi)} & J\frac{k_\parallel}{K} \end{pmatrix},$$

and

$$H^{b,t}_{\text{inter}} = \left(H^{t,b}_{\text{inter}}\right)^\dagger = J\frac{k}{K}e^{-k\Delta z}\begin{pmatrix} e^{i\theta} & -e^{-i(\theta+2\varphi)} \\ -e^{i(\theta+2\varphi)} & e^{-i\theta} \end{pmatrix}.$$

Here, the short-range interlayer e-h exchange interaction has been quenched due to the exponential decay factor $e^{-G\Delta z}$. By assuming that the strain of bottom layer ($l = b$) is along $x$ direction with $\epsilon_{st} = 1\%$, which gives $J^b_0 \approx -6\,\text{meV}$ [2]. So

$$J^t_0 \approx \eta_\theta \eta_{\text{int}} J^b_0 \left(\cos 2\theta + \sin 2\theta\right).$$

In the main text, we have taken $\eta_\theta \equiv 1$ for simplicity, which means

$$J^t_0 \approx \eta_\theta \eta_{\text{int}} J^b_0 \left(\cos 2\theta + \sin 2\theta\right) = J^b_0 \frac{\cos 2\theta + \sin 2\theta}{2}.$$

as shown in Fig. S2(d).

### B. Excitonic Hamiltonian of BP

The excitonic Hamiltonian of BP can be obtained in the basis of $\{|b,\boldsymbol{k}\rangle_\Gamma, |t,\boldsymbol{k}\rangle_\Gamma\}$ by using the same approach as for TMDs. Since there is only one valley ($\alpha, \beta = \Gamma$) per layer under the low-energy approximation, this Hamiltonian takes a simple $2\times 2$ form as

$$H_{\text{BP}} = \begin{pmatrix} \frac{\hbar^2 k_x^2}{2m^{x,b}_{ex,\alpha}} + \frac{\hbar^2 k_y^2}{2m^{y,b}_{ex,\alpha}} & 0 \\ 0 & \frac{\hbar^2 k_x^2}{2m^{x,t}_{ex,\beta}} + \frac{\hbar^2 k_y^2}{2m^{y,t}_{ex,\beta}} \end{pmatrix} + \begin{pmatrix} J^b_\Gamma & J^{b,t}_\Gamma \\ J^{t,b}_\Gamma & J^t_\Gamma \end{pmatrix}, \tag{30}$$

with highly anisotropic effective mass $m^{x,b}_{ex} \approx 0.32m_e$, $m^{y,b}_{ex} \approx 7.47m_e$ and Bohr radius $a^b_{B,x} = \frac{\epsilon_r a_0}{\mu_x/m_e} \approx 29.93\,\text{Å}$, $a^b_{B,y} = \frac{\epsilon_r a_0}{\mu_y/m_e} \approx 2.51\,\text{Å}$ of intralyer excitons in the untwisted layer [20–23]. $\epsilon_r \approx 3$ comes from the environment encapsulating the BP [21, 24]. The similar parameters of the upper layer is with respect to $\theta$. According to Eq. (6), we have

$$\begin{aligned} J^{l=b,t}_\Gamma &\approx \rho^l(0)\frac{V(\boldsymbol{k})}{4}\left|k_+ e^{-i\theta_l} d^-_{cv,\Gamma} + k_- e^{i\theta_l} d^+_{cv,\Gamma}\right|^2 \\ &= \mathcal{J}^l \frac{k}{X}\cos^2(\varphi + \theta_l). \end{aligned} \tag{31}$$

In this case, $\rho^l(0) \sim 1/\left(a^l_{B,x}a^l_{B,y}\right)$, $\boldsymbol{d}_{cv,\Gamma} = (a_x t/\varepsilon, 0)$ according to the single-particle two-band $\boldsymbol{k}\cdot\boldsymbol{p}$ Hamiltonian [20]. $X = \pi/a_x$ is the width of the first Brillouin zone in the $x$ direction. In the main text, we take $a_x = 4.58\,\text{Å}$, $t = 4.862\,\text{eV}$ and $\varepsilon = 2\,\text{eV}$ from the first-principle fitting of the low-energy effective model [20–23], which gives $\mathcal{J}^b \approx 1.09\,\text{eV}$.

$$\begin{aligned} J^{b,t}_{\Gamma} &= J^{t,b}_{\Gamma} \\ &\approx \left[\psi^b_{\Gamma}(0)\right]^* \psi^t_{\Gamma}(0)\, V(\boldsymbol{k},\Delta z)\left(\boldsymbol{k}\cdot\boldsymbol{d}_{cv,\Gamma}\right)\times \\ &\quad \frac{\left(k_+ e^{i\theta} d^-_{cv,\Gamma} + k_- e^{-i\theta} d^+_{cv,\Gamma}\right)^*}{2} \\ &= \sqrt{\mathcal{J}^b\mathcal{J}^t}\frac{k_x}{X}e^{-k\Delta z}\cos(\varphi+\theta). \end{aligned} \tag{32}$$

The excitonic dispersions and eigenstates of $H_{\mathrm{BP}}$ can be formulated as

$$\begin{aligned} \varepsilon_{1,2} = \hbar^2&\left(M^+_x k^2_x + M^+_y k^2_y\right) + \\ &\frac{k}{X}\frac{\mathcal{J}^b\cos^2\varphi + \mathcal{J}^t\cos^2(\varphi+\theta)}{2} \\ &\pm\sqrt{A^2+B^2}, \end{aligned} \tag{33}$$

$$\begin{aligned} |\psi_1\rangle &= \frac{1}{\sqrt{\Omega}}\begin{Bmatrix} A+\sqrt{A^2+B^2} \\ B \end{Bmatrix}, \\ |\psi_2\rangle &= \frac{1}{\sqrt{\Omega}}\begin{Bmatrix} -B \\ A+\sqrt{A^2+B^2} \end{Bmatrix}, \\ \Omega &= 2\sqrt{A^2+B^2}\left(\sqrt{A^2+B^2}+A\right), \end{aligned}$$

here $A = \hbar^2\left(M^-_x k^2_x + M^-_y k^2_y\right) + \frac{k}{X}\frac{\mathcal{J}^b\cos^2\varphi - \mathcal{J}^t\cos^2(\varphi+\theta)}{2}$ and $B = \sqrt{\mathcal{J}^b\mathcal{J}^t}\frac{k}{X}e^{-kz}\cos\varphi\cos(\varphi+\theta)$ are functions of the twist angle $\theta$, with

$$M^{\pm}_x = \frac{m^{x,b}_{ex} \pm m^{x,t}_{ex}}{4m^{x,b}_{ex}m^{x,t}_{ex}}, M^{\pm}_y = \frac{m^{y,b}_{ex} \pm m^{x,t}_{ex}}{4m^{y,b}_{ex}m^{y,t}_{ex}}.$$

Unlike in TMDs, the highly anisotropic feature of the material leads to an $\theta$-dependent excitonic Hamiltonian.

## S2. Derivation of the time-reversal even Hall effect (TREHE)

Here we give a brief introduction about the derivation of the TREHE. Since

$$f_n(\boldsymbol{k}) \approx f^0_n + \delta f^0_n,$$

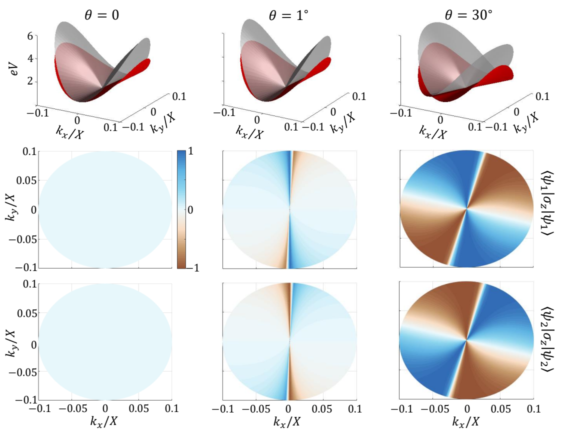


FIG. S3. (color online) Excitonic bands of effective Hamiltonian $H_{BP}$ (Eq. 30) and related layer pseudospin texture $\langle\psi_l|\sigma_z|\psi_l\rangle$ for different values of the twist angle $\theta$.

with

$$f_n^0 = \frac{g_n}{\exp\left(\frac{\varepsilon_n - \mu}{k_B T}\right) - 1},$$

is the Bose-Einstein distribution function, $g_n$ is the degeneracy of the energy level $\varepsilon_n$ and $k_B \approx 8.617 \times 10^{-5}$ eV/K is the Boltzmann constant.

$$\delta f_n^0 = -\tau \frac{df_n^0}{dt} = -\tau \left( \dot{\boldsymbol{x}}_n \cdot \nabla f_n^0 + \hbar \dot{\boldsymbol{k}} \cdot \nabla_{\hbar \boldsymbol{k}} f_n^0 + \partial_t f_n^0 \right),$$

$\dot{\boldsymbol{x}}_n \equiv \boldsymbol{v}_n = \frac{\partial H(\boldsymbol{k})}{\hbar \partial \boldsymbol{k}}$ is the velocity of the $n$th band of the system $H(\boldsymbol{k})$. If we consider the inhomogeneous distribution of the temperature $T$ and the chemical potential $\mu$ in real space, we have

$$\begin{aligned} \delta f_n^0 &= -\tau \frac{df_n^0}{dt} \\ &= -\tau \left( \dot{\boldsymbol{x}}_n \cdot \nabla f_n^0 + \hbar \dot{\boldsymbol{k}} \cdot \nabla_{\hbar \boldsymbol{k}} f_n^0 + \partial_t f_n^0 \right) \\ &\quad -\tau \dot{\boldsymbol{x}} \cdot \left( \partial_T f_n^0 \nabla T + \partial_\mu f_n^0 \nabla \mu \right), \end{aligned}$$

with

$$\nabla f_n^0 = -\frac{\frac{\nabla \varepsilon}{k_B T} \exp\left(\frac{\varepsilon_n - \mu}{k_B T}\right)}{\left[\exp\left(\frac{\varepsilon_n - \mu}{k_B T}\right) - 1\right]^2} = \partial_{\varepsilon_n} f_n^0 \nabla \varepsilon_n, \nabla_{\hbar \boldsymbol{k}} f_n^0 = \partial_{\varepsilon_n} f_n^0 \nabla_{\hbar \boldsymbol{k}} \varepsilon_n, \partial_t f_n^0 = \partial_{\varepsilon_n} f_0^n \partial_t \varepsilon_n,$$

and

$$\partial_T f_n^0 \nabla T = \frac{\frac{\varepsilon_n - \mu}{k_B T^2} \exp\left(\frac{\varepsilon_n - \mu}{k_B T}\right)}{\left[\exp\left(\frac{\varepsilon_n - \mu}{k_B T}\right) - 1\right]^2} \nabla T = \frac{\nabla T}{T} (\varepsilon - \mu) \frac{\frac{1}{k_B T} \exp\left(\frac{\varepsilon_n - \mu}{k_B T}\right)}{\left[\exp\left(\frac{\varepsilon_n - \mu}{k_B T}\right) - 1\right]^2}$$

$$= -\frac{\nabla T}{T} (\varepsilon - \mu) \partial_\varepsilon f_0^n,$$

$$\partial_\mu f_n^0 \nabla \mu = \frac{\frac{1}{k_B T} \exp\left(\frac{\varepsilon_n - \mu}{k_B T}\right)}{\left[\exp\left(\frac{\varepsilon_n - \mu}{k_B T}\right) - 1\right]^2} \nabla \mu = -\nabla \mu \partial_{\varepsilon_n} f_n^0.$$

For excitons which are the neutral particles, there may exists a general force as $\boldsymbol{F} = \hbar \dot{\boldsymbol{k}}$ to induce the current density. In our consideration in the main text, there is no inhomogeneous distribution of $\mu$, also the explicit time dependence, which leads to $\nabla f_n^0 = 0$, $\nabla \mu = 0$, and $\partial_t f_n^0 = 0$. So

$$\delta f_n^0 = -\tau \frac{d f_n^0}{dt} \approx -\tau \left( \hbar \dot{\boldsymbol{k}} \cdot \nabla_{\hbar \boldsymbol{k}} f_n^0 + \dot{\boldsymbol{x}} \cdot \partial_T f_n^0 \nabla T \right) \tag{34}$$

$$= -\frac{\tau}{\hbar} \left( \boldsymbol{F} \cdot \nabla_{\boldsymbol{k}} f_n^0 + \langle u_n(\boldsymbol{k}) | \frac{\partial H_{ex}}{\partial \boldsymbol{k}} | u_n(\boldsymbol{k}) \rangle \cdot \partial_T f_n^0 \nabla T \right).$$

Finally, the transverse current conductivity $\sigma^{\text{sys/env}}$ and Nernst conductivity $\alpha^{\text{sys/env}}$ can be defined as

$$\boldsymbol{j}_{\text{trans}}^{\text{sys/env}} = \sigma^{\text{sys/env}} \boldsymbol{F} + \alpha^{\text{sys/env}} (-k_B \nabla T), \tag{35}$$

with

$$j_{x,\text{trans}}^{\text{sys/env}} = \sigma_{xy}^{\text{sys/env}} F_y + \alpha_{xy}^{\text{sys/env}} (-k_B \partial_y T), j_{y,\text{trans}}^{\text{sys/env}} = \sigma_{yx}^{\text{sys/env}} F_x + \alpha_{yx}^{\text{sys/env}} (-k_B \partial_x T)$$

$$\sigma_{xy}^{\text{sys/env}} \approx -\frac{\tau}{\hbar} \sum_n \int \frac{d^2 \boldsymbol{k}}{(2\pi)^2} \partial_{k_y} f_n^0 v_{x,n}^l(\boldsymbol{k}), \sigma_{yx}^{\text{sys/env}} \approx -\frac{\tau}{\hbar} \sum_n \int \frac{d^2 \boldsymbol{k}}{(2\pi)^2} \partial_{k_x} f_n^0 v_{y,n}^{\text{sys/env}}(\boldsymbol{k}),$$

$$\alpha_{xy}^{\text{sys/env}} \approx \frac{\tau}{\hbar} \frac{1}{k_B T} \sum_n \int \frac{d^2 \boldsymbol{k}}{(2\pi)^2} \langle u_n(\boldsymbol{k}) | \frac{\partial H_{ex}}{\partial k_y} | u_n(\boldsymbol{k}) \rangle (\varepsilon_n - \mu) \partial_{\varepsilon_n} f_n^0 v_{x,n}^{\text{sys/env}}(\boldsymbol{k}),$$

$$\alpha_{yx}^{\text{sys/env}} \approx \frac{\tau}{\hbar} \frac{1}{k_B T} \sum_n \int \frac{d^2 \boldsymbol{k}}{(2\pi)^2} \langle u_n(\boldsymbol{k}) | \frac{\partial H_{ex}}{\partial k_x} | u_n(\boldsymbol{k}) \rangle (\varepsilon_n - \mu) \partial_{\varepsilon_n} f_n^0 v_{y,n}^{\text{sys/env}}(\boldsymbol{k}).$$

This indicates that conductivity of TREHE has the form [25]

$$\sigma_H^{\text{sys/env}} = \frac{\sigma_{xy}^{\text{sys/env}} - \sigma_{yx}^{\text{sys/env}}}{2} = -\frac{\tau}{2\hbar} \sum_n \int \frac{d^2 \boldsymbol{k}}{(2\pi)^2} \left[ \partial_{k_y} f_n^0 v_{x,n}^{\text{sys/env}}(\boldsymbol{k}) - \partial_{k_x} f_n^0 v_{y,n}^{\text{sys/env}}(\boldsymbol{k}) \right]$$

$$= \frac{\tau}{\hbar} \frac{\hbar}{2} \sum_n \int \frac{d^2 \boldsymbol{k}}{(2\pi)^2} \partial_{\varepsilon_n} f_0^n \left[ \boldsymbol{v}_n(\boldsymbol{k}) \times \boldsymbol{v}_n^{\text{sys/env}}(\boldsymbol{k}) \right]$$

$$= -\frac{\tau}{\hbar} \sum_n \int \frac{d^2 \boldsymbol{k}}{(2\pi)^2} f_0^n \frac{\nabla_k \times \boldsymbol{v}_n^{\text{sys/env}}(\boldsymbol{k})}{2}, \tag{36}$$

$$
\begin{aligned}
\alpha_H^{\text{sys/env}} &= \frac{\alpha_{xy}^{\text{sys/env}} - \alpha_{yx}^{\text{sys/env}}}{2} \\
&= \frac{\tau}{\hbar}\frac{\hbar}{2k_BT}\sum_n \int \frac{d^2\boldsymbol{k}}{(2\pi)^2}(\varepsilon_n - \mu)\,\partial_\varepsilon f_0^n \left[v_{y,n}(\boldsymbol{k})\, v_{x,n}^{\text{sys/env}}(\boldsymbol{k}) - v_{x,n}(\boldsymbol{k})\, v_{y,n}^{\text{sys/env}}(\boldsymbol{k})\right] \\
&= -\frac{\tau}{\hbar}\frac{\hbar}{2}\sum_n \int \frac{d^2\boldsymbol{k}}{(2\pi)^2}\frac{\varepsilon_n - \mu}{k_BT}\partial_\varepsilon f_0^n \left[\boldsymbol{v}_n(\boldsymbol{k}) \times \boldsymbol{v}_n^{\text{sys/env}}(\boldsymbol{k})\right] \\
&= \frac{\tau}{\hbar}\sum_n \int \frac{d^2\boldsymbol{k}}{(2\pi)^2}\frac{\varepsilon_n - \mu}{k_BT} f_0^n \frac{\nabla_k \times \boldsymbol{v}_n^{\text{sys/env}}(\boldsymbol{k})}{2}.
\end{aligned}
$$

The relative minus appeared in $\sigma_H^{\text{sys/env}}$ comparing with the previous literature comes from the convention $\sigma_H^{\text{sys/env}} = \left(\sigma_{xy}^{\text{sys/env}} - \sigma_{yx}^{\text{sys/env}}\right)/2$ instead of $\sigma_H^{\text{sys/env}} = \left(\sigma_{yx}^{\text{sys/env}} - \sigma_{xy}^{\text{sys/env}}\right)/2$ using in [25]. The longitudinal conductivity can also be expressed as

$$
\boldsymbol{j}_{\text{long}}^{\text{sys/env}} = \sigma^{\text{sys/env}}\boldsymbol{F} + \alpha^{\text{sys/env}}(-k_B\nabla T), \tag{37}
$$

with

$$
j_{x,\text{long}}^{\text{sys/env}} = \sigma_{xx}^{\text{sys/env}} F_x + \alpha_{xx}^{\text{sys/env}}(-k_B\partial_x T),\, j_{y,\text{long}}^{\text{sys/env}} = \sigma_{yy}^{\text{sys/env}} F_y + \alpha_{yy}^{\text{sys/env}}(-k_B\partial_y T)
$$

$$
\begin{aligned}
\sigma_{xx}^{\text{sys/env}} &\approx -\frac{\tau}{\hbar}\sum_n \int \frac{d^2\boldsymbol{k}}{(2\pi)^2}\partial_{k_x} f_n^0 v_{x,n}^{\text{sys/env}}(\boldsymbol{k}),\, \sigma_{yy}^{\text{sys/env}} \approx -\frac{\tau}{\hbar}\sum_n \int \frac{d^2\boldsymbol{k}}{(2\pi)^2}\partial_{k_y} f_n^0 v_{y,n}^{\text{sys/env}}(\boldsymbol{k}), \\
\alpha_{xx}^{\text{sys/env}} &\approx \frac{\tau}{\hbar}\frac{1}{k_BT}\sum_n \int \frac{d^2\boldsymbol{k}}{(2\pi)^2}\langle u_n(\boldsymbol{k})|\frac{\partial H_{ex}}{\partial k_x}|u_n(\boldsymbol{k})\rangle(\varepsilon_n - \mu)\,\partial_{\varepsilon_n} f_n^0 v_{x,n}^{\text{sys/env}}(\boldsymbol{k}), \\
\alpha_{yy}^{\text{sys/env}} &\approx \frac{\tau}{\hbar}\frac{1}{k_BT}\sum_n \int \frac{d^2\boldsymbol{k}}{(2\pi)^2}\langle u_n(\boldsymbol{k})|\frac{\partial H_{ex}}{\partial k_y}|u_n(\boldsymbol{k})\rangle(\varepsilon_n - \mu)\,\partial_{\varepsilon_n} f_n^0 v_{y,n}^{\text{sys/env}}(\boldsymbol{k}).
\end{aligned}
$$

Here, one can easily find

$$
\begin{aligned}
\sigma_{xy} = \sigma_{xy}^{\text{sys}} + \sigma_{xy}^{\text{env}} &= -\frac{\tau}{\hbar}\sum_n \int \frac{d^2\boldsymbol{k}}{(2\pi)^2}\partial_{k_y} f_n^0 v_{x,n}(\boldsymbol{k}) \\
&= -\tau \sum_n \int \frac{d^2\boldsymbol{k}}{(2\pi)^2}\partial_{\varepsilon_n} f_n^0 \left(\nabla_{\hbar k_y}\varepsilon_n\right) v_{x,n}(\boldsymbol{k}) \\
&= -\tau \sum_n \int \frac{d^2\boldsymbol{k}}{(2\pi)^2}\partial_{\varepsilon_n} f_n^0 v_{y,n}(\boldsymbol{k})\, v_{x,n}(\boldsymbol{k}) \\
&= \sigma_{yx}^{\text{sys}} + \sigma_{yx}^{\text{env}} = \sigma_{yx},
\end{aligned} \tag{38}
$$

the similar process gives

$$
\alpha_{xy} = \alpha_{xy}^{\text{sys}} + \alpha_{xy}^{\text{env}} = \alpha_{yx}^{\text{sys}} + \alpha_{yx}^{\text{env}} = \alpha_{yx}, \tag{39}
$$

which means

$$\sigma_H^{\text{sys}} = \frac{\sigma_{xy}^{\text{sys}} - \sigma_{yx}^{\text{sys}}}{2} = \frac{\sigma_{yx}^{\text{env}} - \sigma_{xy}^{\text{env}}}{2} = -\sigma_H^{\text{env}},$$
$$\alpha_H^{\text{sys}} = \frac{\alpha_{xy}^{\text{sys}} - \alpha_{yx}^{\text{sys}}}{2} = \frac{\alpha_{yx}^{\text{env}} - \alpha_{xy}^{\text{env}}}{2} = -\alpha_H^{\text{env}}. \tag{40}$$

## S3. Derivation of the crossed nonlinear dynamical Hall effect (CNDHE)

According to the previous theoretical works [26–28], we can apply the related calculations directly to the excitonic system. If there is an out-of-plane mechanical force $F_\perp = F_\perp^0 f(t)$ in the system, the Hamiltonian can be with respect to time $t$ explicitly. The current density of excitons in the intrinsic response can be given as [29, 30]

$$\boldsymbol{j} = \sum_n \int \frac{d^2\boldsymbol{k}}{(2\pi)^2} f_n^0(\boldsymbol{k})\, \boldsymbol{v}_n(\boldsymbol{k}) + \nabla \times \boldsymbol{M}(r),$$

where

$$\boldsymbol{v}_n(\boldsymbol{k}) = \frac{\partial \varepsilon_n(\boldsymbol{k})}{\hbar \partial \boldsymbol{k}} + \dot{F}_\perp \boldsymbol{\Omega}_{n,F_\perp \boldsymbol{k}} - \frac{d\boldsymbol{k}}{dt} \times \boldsymbol{\Omega}_{n,\boldsymbol{k}},$$
$$\boldsymbol{M}(r) = \frac{k_B T}{\hbar} \sum_n \int \frac{d^2\boldsymbol{k}}{(2\pi)^2} \boldsymbol{\Omega}_{n,\boldsymbol{k}} \log\left(1 - e^{-(\varepsilon_n - \mu)/k_B T}\right). \tag{41}$$

Here $\boldsymbol{F}_\parallel = \hbar \frac{d\boldsymbol{k}}{dt}$ represents the in-plane mechanical force, $\boldsymbol{\Omega}_{n,\boldsymbol{k}} = \Omega_{n,k_x k_y} \hat{e}_z$ is the Berry curvature of excitons in momentum space, and the velocity $\boldsymbol{v}_n(\boldsymbol{k})$ is only expanded into the first order of $F_\perp \left(\dot{F}_\perp\right)$ and $\boldsymbol{F}_\parallel$.

$$\begin{aligned}
\nabla \times \boldsymbol{M}(r) &= \frac{k_B}{\hbar} \nabla T \times \sum_n \int \frac{d^2\boldsymbol{k}}{(2\pi)^2} \boldsymbol{\Omega}_{n,\boldsymbol{k}} \log\left[1 - e^{-(\varepsilon_n - \mu)/k_B T}\right] \\
&+ \frac{k_B T}{\hbar} \nabla T \times \sum_n \int \frac{d^2\boldsymbol{k}}{(2\pi)^2} \boldsymbol{\Omega}_{n,\boldsymbol{k}} \frac{-e^{-(\varepsilon_n - \mu)/k_B T}}{1 - e^{-(\varepsilon_n - \mu)/k_B T}} \frac{\varepsilon_n - \mu}{k_B T^2} \\
&+ \frac{k_B T}{\hbar} \nabla \mu \times \sum_n \int \frac{d^2\boldsymbol{k}}{(2\pi)^2} \boldsymbol{\Omega}_{n,\boldsymbol{k}} \frac{-e^{-(\varepsilon_n - \mu)/k_B T}}{1 - e^{-(\varepsilon_n - \mu)/k_B T}} \frac{1}{k_B T} \\
&= -\frac{\nabla \mu}{\hbar} \times \sum_n \int \frac{d^2\boldsymbol{k}}{(2\pi)^2} f_n^0(\boldsymbol{k})\, \boldsymbol{\Omega}_{n,\boldsymbol{k}} - \\
&\quad \frac{\nabla T}{\hbar T} \times \sum_n \int \frac{d^2\boldsymbol{k}}{(2\pi)^2} \boldsymbol{\Omega}_{n,\boldsymbol{k}} \left[(\varepsilon_n - \mu) f_n^0(\boldsymbol{k}) - k_B T \log\left(1 - e^{-(\varepsilon_n - \mu)/k_B T}\right)\right],
\end{aligned}$$

if the inhomogeneous distribution of the temperature $T$ and chemical potential $\mu$ appears in real space. Due to the existence of the time-reversal symmetry and at least the $C_2$ symmetry

(or other higher rotational symmetries), just let $H_0 = H_{ex}(\boldsymbol{k})$ with $F_\perp^0 = 0$ and $\boldsymbol{F}_\parallel = 0$, the previous literature prove that [26–28]

$$\varepsilon_n(\boldsymbol{k}) \approx \varepsilon_n^0(\boldsymbol{k}) - \dot{F}_\perp \frac{d\boldsymbol{k}}{dt} \cdot \mathcal{G}^n(\boldsymbol{k}), \tag{42}$$

where $H_0 |u_n^0\rangle = \varepsilon_n^0(\boldsymbol{k}) |u_n^0\rangle$ in the zero order of $F_\perp \left(\dot{F}_\perp\right)$ and $\boldsymbol{F}_\parallel$, the second term comes from the perturbation part of the energy, which is in the order of $\dot{F}_\perp \boldsymbol{F}_\parallel$ and

$$\mathcal{G}^n(\boldsymbol{k}) = 2\hbar^2 \mathrm{Re} \sum_{m \neq n} \frac{\langle u_n^0 | p_z | u_m^0 \rangle}{(\varepsilon_n^0 - \varepsilon_m^0)^3} \boldsymbol{v}_{mn}^0, \tag{43}$$

is the $\boldsymbol{k}$-space curl of the interlayer Berry connection polarizability (BCP) [26]. The hybrid Berry curvature $\boldsymbol{\Omega}_{n,F_\perp \boldsymbol{k}}$ in the $(F_\perp, \boldsymbol{k})$ space with the first order of $\boldsymbol{F}_\parallel$ is given as

$$\begin{aligned} \boldsymbol{\Omega}_{n,F_\perp \boldsymbol{k}} &= -\left(\frac{\partial \mathcal{A}_{F_\perp}}{\partial \boldsymbol{k}} - \frac{\partial \mathcal{A}_{\boldsymbol{k}}^{F_\perp}}{\partial F_\perp}\right) \\ &\approx \partial \frac{\mathcal{A}_{\boldsymbol{k}}^{0,F_\perp} + \mathcal{A}_{\boldsymbol{k}}^{\boldsymbol{F}_\parallel, F_\perp}}{\partial F_\perp} - \partial \frac{\mathcal{A}_{F_\perp}^0 + \mathcal{A}_{F_\perp}^{\boldsymbol{F}_\parallel}}{\partial \boldsymbol{k}}, \end{aligned} \tag{44}$$

where $\mathcal{A}_{\boldsymbol{k}}^{0,F_\perp} \equiv \langle u_n | \frac{\partial}{\partial \boldsymbol{k}} | u_n \rangle$ is the Berry connection of $\boldsymbol{k}$ that only includes the first order of $F_\perp$, while $\mathcal{A}_{\boldsymbol{k}}^{\boldsymbol{F}_\parallel, F_\perp}$ includes the first order of $F_\perp$ and $\boldsymbol{F}_\parallel$. $\mathcal{A}_{F_\perp}^0 \equiv \langle u_n | \frac{\partial}{\partial F_\perp} | u_n \rangle$ is the Berry connection of $F_\perp$ in the zero order of $F_\perp$ and $\boldsymbol{F}_\parallel$, while $\mathcal{A}_{F_\perp}^{\boldsymbol{F}_\parallel}$ only contains the first order of $\boldsymbol{F}_\parallel$, respectively.

In general, we have

$$\begin{aligned} \mathcal{A}_{F_\perp}^0(\boldsymbol{k}) &= i \langle u_n | \frac{\partial}{\partial F_\perp} | u_n \rangle_{\boldsymbol{F}_\parallel = 0, F_\perp = 0} \\ &= i \langle u_n(\boldsymbol{k}) | \mathcal{T}^\dagger \frac{\partial}{\partial F_\perp} \mathcal{T} | u_n(\boldsymbol{k}) \rangle \\ &= i \langle u_n(-\boldsymbol{k}) |^* \frac{\partial}{\partial F_\perp} | u_n(-\boldsymbol{k}) \rangle^* \\ &= -i \langle u_n(-\boldsymbol{k}) | \frac{\partial}{\partial F_\perp} | u_n(-\boldsymbol{k}) \rangle = -\mathcal{A}_{F_\perp}^0(-\boldsymbol{k}), \end{aligned} \tag{45}$$

because of the time-reversal symmetry $\mathcal{T}$ and

$$\begin{aligned} \mathcal{A}_{F_\perp}^0(\boldsymbol{k}) &= i \langle u_n | \frac{\partial}{\partial F_\perp} | u_n \rangle_{\boldsymbol{F}_\parallel = 0, F_\perp = 0} \\ &= i \langle u_n(\boldsymbol{k}) | \mathcal{C}_n^{-1} \frac{\partial}{\partial F_\perp} \mathcal{C}_n | u_n(\boldsymbol{k}) \rangle \\ &= i \langle u_n(\mathcal{C}_n \boldsymbol{k}) | \frac{\partial}{\partial F_\perp} | u_n(\mathcal{C}_n \boldsymbol{k}) \rangle = \mathcal{A}_{F_\perp}^0(\mathcal{C}_n \boldsymbol{k}), \end{aligned} \tag{46}$$

due to the rotational symmetry $\mathcal{C}_n$. If $n$ is even number, $\mathcal{A}^0_{F_\perp}(\boldsymbol{k}) = \mathcal{A}^0_{F_\perp}(-\boldsymbol{k})$ can always satisfy, leading to $\mathcal{A}^0_{F_\perp}(\boldsymbol{k}) = 0$. For $n$ is odd, it is easy to prove that $\int \frac{d^2\boldsymbol{k}}{(2\pi)^2}\frac{\partial \mathcal{A}^0_{F_\perp}}{\partial \boldsymbol{k}} = 0$. Also

$$\begin{aligned}
\mathcal{A}^{0,F_\perp}_{\boldsymbol{k}} &= i\left\langle u_n^1\right| \frac{\partial}{\partial \boldsymbol{k}}\left|u_n^1\right\rangle_{\boldsymbol{F}_\parallel=0} \\
&= i\left\langle u_n^1(\boldsymbol{k})\right| \mathcal{T}^\dagger \frac{\partial}{\partial \boldsymbol{k}}\mathcal{T}\left|u_n^1(\boldsymbol{k})\right\rangle \\
&= i\left\langle u_n^1(-\boldsymbol{k})\right|^* \frac{\partial}{\partial \boldsymbol{k}}\left|u_n^1(-\boldsymbol{k})\right\rangle^* \\
&= -i\left\langle u_n^1(-\boldsymbol{k})\right| \frac{\partial}{\partial \boldsymbol{k}}\left|u_n^1(-\boldsymbol{k})\right\rangle = \mathcal{A}^{0,F_\perp}_{-\boldsymbol{k}}, \\
\mathcal{A}^{0,F_\perp}_{\boldsymbol{k}} &= i\left\langle u_n^1\right| \frac{\partial}{\partial \boldsymbol{k}}\left|u_n^1\right\rangle_{\boldsymbol{F}_\parallel=0} \\
&= i\left\langle u_n^1(\boldsymbol{k})\right| \mathcal{C}_n^{-1} \frac{\partial}{\partial \boldsymbol{k}}\mathcal{C}_n\left|u_n^1(\boldsymbol{k})\right\rangle \\
&= i\left\langle u_n^1(\mathcal{C}_n\boldsymbol{k})\right| \frac{\partial}{\partial \boldsymbol{k}}\left|u_n^1(\mathcal{C}_n\boldsymbol{k})\right\rangle \\
&= i\left\langle u_n^1(\mathcal{C}_n\boldsymbol{k})\right| \frac{\partial(\mathcal{C}_n\boldsymbol{k})}{\partial \boldsymbol{k}}\frac{\partial}{\partial(\mathcal{C}_n\boldsymbol{k})}\left|u_n^1(\mathcal{C}_n\boldsymbol{k})\right\rangle \\
&= \mathcal{C}_n^{-1}\mathcal{A}^{0,F_\perp}_{\mathcal{C}_n\boldsymbol{k}},
\end{aligned} \tag{47}$$

resulting in $\int \frac{d^2\boldsymbol{k}}{(2\pi)^2}\frac{\partial \mathcal{A}^{0,F_\perp}_{\boldsymbol{k}}}{\partial F_\perp} = 0$. Since [27, 28]

$$\begin{aligned}
&\frac{\partial \varepsilon_n}{\hbar\partial \boldsymbol{k}} - \dot{F}_\perp \frac{\partial \mathcal{A}_{F_\perp}}{\partial \boldsymbol{k}} \\
\approx &\frac{\partial \varepsilon_n^0}{\hbar\partial \boldsymbol{k}} - \dot{F}_\perp \frac{d\boldsymbol{k}}{dt}\cdot\frac{\partial \mathcal{G}^n(\boldsymbol{k})}{\hbar\partial \boldsymbol{k}} - \dot{F}_\perp \frac{\partial \mathcal{A}^0_{F_\perp}}{\partial \boldsymbol{k}} - \dot{F}_\perp \frac{\partial \mathcal{A}^{\boldsymbol{F}_\parallel}_{F_\perp}}{\partial \boldsymbol{k}} \\
= &\frac{\partial \varepsilon_n^0}{\hbar\partial \boldsymbol{k}} - \dot{F}_\perp \frac{\partial \mathcal{A}^0_{F_\perp}}{\partial \boldsymbol{k}},
\end{aligned} \tag{48}$$

due to

$$\dot{F}_\perp \frac{d\boldsymbol{k}}{dt}\cdot\frac{\partial \mathcal{G}^n(\boldsymbol{k})}{\hbar\partial \boldsymbol{k}} + \dot{F}_\perp \frac{\partial \mathcal{A}^{\boldsymbol{F}_\parallel}_{F_\perp}}{\partial \boldsymbol{k}} = 0,$$

and $\mathcal{A}^{\boldsymbol{F}_\parallel,F_\perp}_{\boldsymbol{k}}$ has no contribution to the Hall current, we approximately have

$$\frac{\partial \varepsilon_n(\boldsymbol{k})}{\hbar\partial \boldsymbol{k}} + \dot{F}_\perp \boldsymbol{\Omega}_{n,F_\perp\boldsymbol{k}} \approx 0. \tag{49}$$

Meanwhile

$$\boldsymbol{\Omega}_{\boldsymbol{k}} = \nabla_{\boldsymbol{k}} \times \mathcal{A}_{\boldsymbol{k}} \approx \nabla_{\boldsymbol{k}} \times \left(\mathcal{A}^0_{\boldsymbol{k}} + \mathcal{A}^{\dot{F}_\perp}_{\boldsymbol{k}}\right),$$

Here $\mathcal{A}^{\dot{F}_\perp}_{\boldsymbol{k}} \equiv \langle u_n| \frac{\partial}{\partial \boldsymbol{k}} |u_n\rangle$ is the Berry connection of $\boldsymbol{k}$ that only includes the first order of

$F_\perp\left(\dot{F}_\perp\right)$, which has the form

$$\mathcal{A}_{\boldsymbol{k}}^{\dot{F}_\perp} = -2\hbar^2\dot{F}_\perp \mathrm{Re}\sum_{m\neq n}\frac{\langle u_n^0|\,\frac{\partial H}{\partial F_\perp}\,|u_m^0\rangle}{\left(\varepsilon_n^0-\varepsilon_m^0\right)^3}\langle u_m^0|\,\frac{\partial H}{\hbar\partial\boldsymbol{k}}\,|u_n^0\rangle \tag{50}$$
$$= -\dot{F}_\perp 2\hbar^2\mathrm{Re}\sum_{m\neq n}\frac{\langle u_n^0|\,p_z\,|u_m^0\rangle}{\left(\varepsilon_n^0-\varepsilon_m^0\right)^3}\boldsymbol{v}_{mn}^0 = -\dot{F}_\perp\mathcal{G}^n\left(\boldsymbol{k}\right),$$

The first term has zero contribution after integral since the time-reversal symmetry requires

$$\boldsymbol{\Omega}_{n,\boldsymbol{k}}^0 = \nabla_{\boldsymbol{k}}\times\mathcal{A}_{\boldsymbol{k}}^0 = -\boldsymbol{\Omega}_{n,-\boldsymbol{k}}^0,$$

then finally we have

$$\boldsymbol{v}_n\left(\boldsymbol{k}\right)\approx-\frac{d\boldsymbol{k}}{dt}\times\left(\nabla_{\boldsymbol{k}}\times\mathcal{A}_{\boldsymbol{k}}^{\dot{F}_\perp}\right), \tag{51}$$

if we only consider the Hall current. The related Hall current can be represented as

$$j_{x,H} = \sigma_{xy}\left(F_y+\nabla_y\mu\right)+\alpha_{xy}\left(-k_B\partial_yT\right), j_{y,H} = \sigma_{yx}\left(F_x+\nabla_x\mu\right)+\alpha_{yx}\left(-k_B\partial_xT\right), \tag{52}$$

$$\sigma_H = \sigma_{xy} = -\frac{1}{\hbar}\sum_n\int\frac{d^2\boldsymbol{k}}{\left(2\pi\right)^2}f_n^0\left(\boldsymbol{k}\right)\left(\nabla_{\boldsymbol{k}}\times\mathcal{A}_{\boldsymbol{k}}^{\dot{F}_\perp}\right) = -\sigma_{yx},$$
$$\alpha_H = \alpha_{xy}$$
$$= \frac{1}{\hbar T}\sum_n\int\frac{d^2\boldsymbol{k}}{\left(2\pi\right)^2}\left(\nabla_{\boldsymbol{k}}\times\mathcal{A}_{\boldsymbol{k}}^{\dot{F}_\perp}\right)\left[\frac{\varepsilon_n-\mu}{k_B}f_n^0\left(\boldsymbol{k}\right)-T\log\left(1-e^{-\left(\varepsilon_n-\mu\right)/k_BT}\right)\right]$$
$$= -\alpha_{yx}.$$

Assuming that $F_\perp = F_\perp^0 f\left(t\right) = F_\perp^0\cos\left(\omega t\right)$ and $|u_n\rangle\equiv|u_n^0\rangle$ as we used in the main text, it shows

$$\sigma_H = -\frac{1}{\hbar}\sum_n\int\frac{d^2\boldsymbol{k}}{\left(2\pi\right)^2}f_n^0\left(\boldsymbol{k}\right)\left(\nabla_{\boldsymbol{k}}\times\mathcal{A}_{\boldsymbol{k}}^{\dot{F}_\perp}\right)$$
$$= -F_\perp^0\omega\sin\left(\omega t\right)\frac{1}{\hbar}\sum_n\int\frac{d^2\boldsymbol{k}}{\left(2\pi\right)^2}f_n^0\left(\boldsymbol{k}\right)\left(\nabla_{\boldsymbol{k}}\times\mathcal{G}^n\left(\boldsymbol{k}\right)\right),$$
$$\alpha_H = \frac{F_\perp^0\omega\sin\left(\omega t\right)}{\hbar}\times$$
$$\sum_n\int\frac{d^2\boldsymbol{k}}{\left(2\pi\right)^2}\left(\nabla_{\boldsymbol{k}}\times\mathcal{G}^n\left(\boldsymbol{k}\right)\right)\left[\frac{\varepsilon_n-\mu}{k_BT}f_n^0\left(\boldsymbol{k}\right)-\log\left(1-e^{-\left(\varepsilon_n-\mu\right)/k_BT}\right)\right].$$

Defining

$$\chi^{\mathrm{int}} = \frac{1}{\hbar}\sum_n\int\frac{d^2\boldsymbol{k}}{\left(2\pi\right)^2}f_n^0\left(\boldsymbol{k}\right)\left(\nabla_{\boldsymbol{k}}\times\mathcal{G}^n\left(\boldsymbol{k}\right)\right),$$
$$\chi_{\mathrm{Ner}}^{\mathrm{int}} = \sum_n\int\frac{d^2\boldsymbol{k}}{\left(2\pi\right)^2}\left(\nabla_{\boldsymbol{k}}\times\mathcal{G}^n\left(\boldsymbol{k}\right)\right)\left[\frac{\varepsilon_n-\mu}{k_BT}f_n^0\left(\boldsymbol{k}\right)-\log\left(1-e^{-\left(\varepsilon_n-\mu\right)/k_BT}\right)\right],$$

it gives the expression of Eq. (13) in the main text.

---


[1] H. Yu, X. Cui, X. Xu, and W. Yao, Valley excitons in two-dimensional semiconductors, Natl. Sci. Rev. **2**, 57-70 (2015).

[2] H. Yu, G. Liu, P. Gong, X. Xu and W. Yao, Dirac cones and Dirac saddle points of bright excitons in monolayer transition metal dichalcogenides, Nat. Commun. **5**, 3876 (2014).

[3] Diana Y. Qiu, Ting Cao, and Steven G. Louie, Nonanalyticity, Valley quantum phases, and lightlike exciton dispersion in monolayer transition metal dichalcogenides: theory and first-principles calculations, Phys. Rev. Lett. **115**, 176801 (2015).

[4] Ci Li and Wang Yao, Cross-dimensional valley excitons from Förster coupling in arbitrarily twisted stacks of monolayer semiconductors, 2D. Mater. **11**, 015006 (2023).

[5] J. Z. Zhang and J. Z. Ma, Two-dimensional excitons in monolayer transition metal dichalcogenides from radial equation and variational calculations, J. Phys.: Condens. Matter **31**, 105702 (2019).

[6] D. Xiao, G.-B. Liu, W. Feng, X. Xu, and W. Yao, Coupled spin and valley physics in monolayers of MoS2 and other group VI dichalcogenides, Phys. Rev. Lett. **108**, 196802 (2012).

[7] Th. Forster, Energiewanderung und Fluoreszenz, Naturwissenschaften **33**, 166–175 (1946).

[8] Bing Shen Wang and Joseph L. Birman, Exciton dispersion in multiple quantum wells and superlattices: An additional contribution to the linewidth, Phys. Rev. B **43**, 12458 (1990).

[9] Judith F. Specht, Andreas Knorr, and Marten Richter, Two-dimensional spectroscopy: An approach to distinguish Förster and Dexter transfer processes in coupled nanostructures, Phys. Rev. B **91**, 155313 (2015).

[10] M. Selig, E. Malic, K. J. Ahn, N. Koch, and A. Knorr, Theory of optically induced Förster coupling in van der Waals coupled heterostructures, Phys. Rev. B **99**, 035420 (2019).

[11] N. S. Rytova, Screened potential of a point charge in a thin film, Proc. MSU, Phys. Astron. **3**, 30 (1967).

[12] L. V. Keldysh, Coulomb interaction in thin semiconductor and semimetal films, JETP Lett. **29**, 658 (1979).

[13] M. Danovich, D. A. Ruiz-Tijerina, R. J. Hunt, M. Szyniszewski, N. D. Drummond, and V. I. Fal'ko, Localized interlayer complexes in heterobilayer transition metal dichalcogenides, Phys.

Rev. B. **97**, 195452 (2018).

[14] D. Y. Qiu, F. H. da Jornada, and S. G. Louie, Optical spectrum of MoS2: many-body effects and diversity of exciton states, Phys. Rev. Lett. **111**, 216805 (2013).

[15] Hemant Kumar, Liang Dong, and Vivek B. Shenoy, Limits of Coherency and Strain Transfer in Flexible 2D van der Waals Heterostructures: Formation of Strain Solitons and Interlayer Debonding, Sci. Rep **6**, 21516 (2016).

[16] Jenny Hu, Leo Yu, Xueqi Chen, Wanhee Lee, C. Mathew Mate, and Tony F. Heinz, Moiré-Assisted Strain Transfer in Vertical van der Waals Heterostructures, Nano. Lett. **23**, 10051-10057 (2023).

[17] B. Amorim, et al, Novel effects of strains in graphene and other two dimensional materials, Phys. Rep. **617**, 1-54 (2016).

[18] Zhen Bi, Noah F. Q. Yuan, and Liang Fu, Designing flat bands by strain, Phys. Rev. B **100**, 035448 (2019).

[19] Huiyuan Zheng, Dawei Zhai, and Wang Yao, Anomalous Magneto-Optical Response and Chiral Interface of Dipolar Excitons at Twisted Valleys, Nano. Lett. **22**, 5466-5472 (2022).

[20] A. S. Rodin, A. Carvalho, and A. H. Castro Neto, Strain-Induced Gap Modification in Black Phosphorus, Phys. Rev. Lett. **112**, 176801 (2014).

[21] Andres Castellanos-Gomez, et. al, Isolation and characterization of few-layer black phosphorus, 2D. Mat. **1**, 025001 (2014).

[22] Jingsi Qiao, Xianghua Kong, Zhi-Xin Hu, Feng Yang, and Wei Ji, High-mobility transport anisotropy and linear dichroism in few-layer black phosphorus, Nat. Commun. **5**, 4475 (2014).

[23] Vy Tran, Ryan Soklaski, Yufeng Liang, and Li Yang, Layer-controlled band gap and anisotropic excitons in few-layer black phosphorus, Phys. Rev. B **89**, 235319 (2014).

[24] Akash Laturia, Maarten L. Van de Put, and William G. Vandenberghe, Dielectric properties of hexagonal boron nitride and transition metal dichalcogenides: from monolayer to bulk, npj 2D Mater Appl **2**, 6 (2018).

[25] Dawei Zhai, Cong Chen, Cong Xiao, and Wang Yao, Time-reversal even charge hall effect from twisted interface coupling, Nat. Commun. **14**, 1961 (2023).

[26] Cong Chen, Dawei Zhai, Cong Xiao, and Wang Yao, Crossed Nonlinear Dynamical Hall Effect in Twisted Bilayers, Phys. Rev. Res **6**, L012059 (2024).

[27] C. Xiao, H. Liu, J. Zhao, S. A. Yang, and Q. Niu, Thermoelectric generation of orbital

magnetization in metals, Phys. Rev. B **103**, 045401 (2021).

[28] C. Xiao, H. Liu, W. Wu, H. Wang, Q. Niu, and S. A. Yang, Intrinsic Nonlinear Electric Spin Generation in Centrosymmetric Magnets, Phys. Rev. Lett. **129**, 086602 (2022).

[29] Di Xiao, Yugui Yao, Zhong Fang, and Qian Niu, Berry-Phase Effect in Anomalous Thermoelectric Transport, Phys. Rev. Lett. **97**, 026603 (2006).

[30] Wang Yao and Qian Niu, Berry Phase Effect on the Exciton Transport and on the Exciton Bose-Einstein Condensate, Phys. Rev. Lett. **101**, 106401 (2008).
